# Supplementary material for: JRDB-PanoTrack: An Open-world Panoptic Segmentation and Tracking Robotic Dataset in Crowded Human Environments
Source: arXiv:2404.01686 source file (2024-04-02)
Supplement: Supplementary file 1 [file X_suppl.tex]

\clearpage
\setcounter{page}{1}
\maketitlesupplementary

% \section{More Analysis}
% \label{sec:rationale}
% %
% Having the supplementary compiled together with the main paper means that:
% %
% \begin{itemize}
% \item The supplementary can back-reference sections of the main paper, for example, we can refer to \cref{sec:intro};
% \item The main paper can forward reference sub-sections within the supplementary explicitly (e.g. referring to a particular experiment);
% \item When submitted to arXiv, the supplementary will already included at the end of the paper.
% \end{itemize}
% %
% To split the supplementary pages from the main paper, you can use \href{https://support.apple.com/en-ca/guide/preview/prvw11793/mac#:~:text=Delete%20a%20page%20from%20a,or%20choose%20Edit%20%3E%20Delete).}{Preview (on macOS)}, \href{https://www.adobe.com/acrobat/how-to/delete-pages-from-pdf.html#:~:text=Choose%20%E2%80%9CTools%E2%80%9D%20%3E%20%E2%80%9COrganize,or%20pages%20from%20the%20file.}{Adobe Acrobat} (on all OSs), as well as \href{https://superuser.com/questions/517986/is-it-possible-to-delete-some-pages-of-a-pdf-document}{command line tools}.

\section{More Experiments}

\textbf{Results of Various Mask Scales.} 
% To further explore the challenges posed by JRDB-Panotrack, we report the OSPA results for objects of three different scales, as defined in \cref{fig:mask_size_per_split}. The CW and OW results are detailed in \cref{tab:cw_ospa_per_scale} and \cref{tab:ow_ospa_per_scale}, respectively. Current methods show a significant performance variation among different scales, struggling with small-scale objects while achieving better results for large-scale objects. This variability in scale is attributed to the dynamic scenes in JRDB-Panotrack, presenting a notable challenge for environment understanding.
The OSPA results for small, medium, and large objects in JRDB-Panotrack (defined in \cref{fig:mask_size_per_split}) reveal significant performance differences across scales. The results for CW and OW are in \cref{tab:cw_ospa_per_scale} and \cref{tab:ow_ospa_per_scale}, respectively. Current methods excel with large-scale objects but struggle with smaller ones, highlighting the challenge of dynamic scene interpretation in JRDB-Panotrack.

% \textbf{3D CW Panoptic Segmentation.} This section delves into the evaluation of SOTA methods in 3D closed-world panoptic segmentation and tracking. Leveraging the correlation between 2D and 3D data, we projected 2D panoptic labels onto 3D point clouds, using these projections as pseudo-labels for model training.
% For evaluation, we use our proposed OSPA and adopt popular metrics for 3D panoptic segmentation (PQ, IOU) and tracking (LSTQ\cite{aygun20214d}). It's important to note that these 3D pseudo-labels may contain noise, potentially affecting result accuracy. In terms of 3D panoptic segmentation, as shown in \cref{tab:3Dclosedworld}, MaskPLS emerges as the superior method, excelling in all metrics. This indicates MaskPLS's enhanced ability to identify and segment objects precisely in 3D space. In 3D panoptic tracking, Mask4D takes the lead in LSTQ\cite{aygun20214d} and achieves the best OSPA score of 0.860, denoting its strength in maintaining object identities and tracking consistency over time. A notable observation here is the higher $S_{assoc}$ scores compared to $S_{cls}$, suggesting that these methods are better at object association and tracking than at precise classification in a 3D environment.\\
%  \vspace{-2em}
%Adapting from the 43 classes in the 2D closed-world setting, we further merge similar or indistinguishable classes in 3D point cloud, resulting in a refined set of 21 classes for our 3D experiments. 
\section{More Statistics and information}

\textbf{Visualization.} %Our annotations are visualised in \cref{fig:stacked_images}, displaying a rich diversity of settings that span both indoor and outdoor environments. These scenes are characterized by a range of lighting conditions, varying degrees of human clsuter, and a variety of dynamic activities. The locations include roads, malls, sidewalks, restaurants, plazas, parks, halls, classrooms, laboratories, and office buildings. In addition, our labeling scheme distinguishes between different floors and objects behind glass or being hung on wall (marked as striped areas), enhancing the understanding of real-world robot scene understanding. This detailed annotation approach is crucial for improving human-robot interactions and aidiOur annotations are visualised in \cref{fig:stacked_images}, displaying a rich diversity of settings that span both indoor and outdoor environments. These scenes are characterized by a range of lighting conditions, varying degrees of human clsuter, and a variety of dynamic activities. The locations include roads, malls, sidewalks, restaurants, plazas, parks, halls, classrooms, laboratories, and office buildings. In addition, our labeling scheme distinguishes between different floors and objects behind glass or being hung on wall (marked as striped areas), enhancing the understanding of real-world robot scene understanding. This detailed annotation approach is crucial for improving human-robot interactions and aiding in robotic decision-making processes.ng in robotic decision-making processes.
Our annotations are visualized in \cref{fig:stacked_images}, displaying a rich diversity of settings that span both indoor and outdoor environments. These images illustrate the versatility of JRDB-PanoTrack, featuring a variety of lighting conditions, varying crowd densities, and diverse human activities. Additionally, \cref{fig:stacked_images} highlights our labeling approach, marking different floors and objects behind glass or on walls with striped areas. This detail is crucial for improving human-robot interaction and decision-making in robotics.
%This detailed annotation approach is crucial for improving human-robot interactions and aiding in robotic decision-making processes.

%\textbf{3D CW Panoptic Segmentation.} This section delves into the evaluation of state-of-the-art methods in 3D closed-world panoptic segmentation and tracking. Leveraging the correlation between 2D and 3D data, we projected 2D panoptic labels onto 3D point clouds, using these projections as pseudo-labels for model training. Adapting from the 43 classes in the 2D closed-world setting, we further merge similar or indistinguishable classes in 3D point cloud, resulting in a refined set of 21 classes for our 3D experiments. For evaluation, we use our proposed OSPA and adopt polular metrics for 3D panoptic segmentation (PQ, IOU) and tracking (LSTQ). It's important to note that these 3D pseudo-labels may contain noise, potentially affecting result accuracy. In terms of 3D panoptic segmentation, as shown in \cref{tab:3Dclosedworld}, MaskPLS emerges as the superior method, excelling in all metrics. This indicates MaskPLS's enhanced ability to identify and segment objects precisely in 3D space. In 3D panoptic tracking, Mask4D takes the lead in LSTQ and achieves the best OSPA score of 0.860, denoting its strength in maintaining object identities and tracking consistency over time. A notable observation here is the higher $S_{assoc}$ scores compared to $S_{cls}$, suggesting that these methods are better at object association and tracking than at precise classification in a 3D environment.

 \begin{figure}[h]
     \centering
     \includegraphics[width=\linewidth]{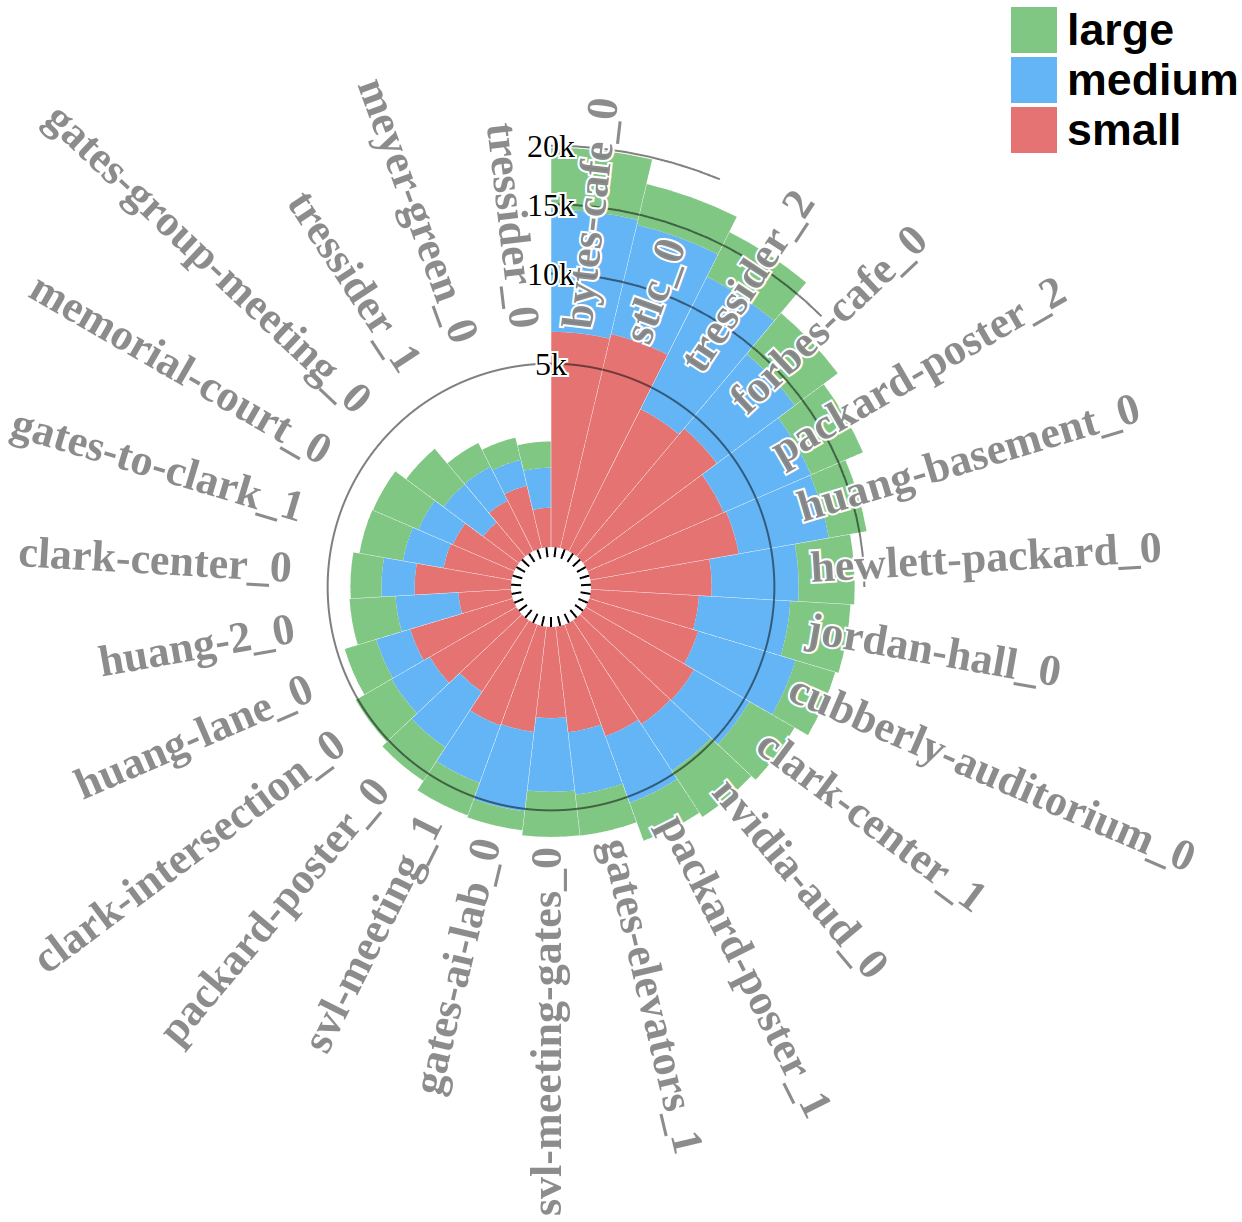}
     \caption{The distribution of mask sizes per sequence in the JRDB-PanoTrack training set.}
     \label{fig:mask_size_per_seq}
 \end{figure}

\noindent\textbf{Detailed Mask size.} Beyond the general mask size trends in JRDB-PanoTrack (\cref{fig:mask_size_per_split}), we also examine the distribution per sequence (\cref{fig:mask_size_per_seq}). 
Masks are categorized by area M: small ($<32^2$), medium ($32^2 < M \leq 96^2$), and large ($>96^2$).
\cref{fig:mask_size_per_seq} shows that the mask size distribution varies notably between indoor and outdoor sequences. Indoor sequences feature a larger quantity of masks, predominantly smaller in size, due to the crowded nature and presence of numerous small objects like chairs, tables, and people. In contrast, outdoor sequences have fewer, but larger masks, reflecting the less crowded spaces with larger 'stuff' classes, such as trees and buildings.

% \begin{figure}[!t]
%     \centering
%     \includegraphics[width=\linewidth]{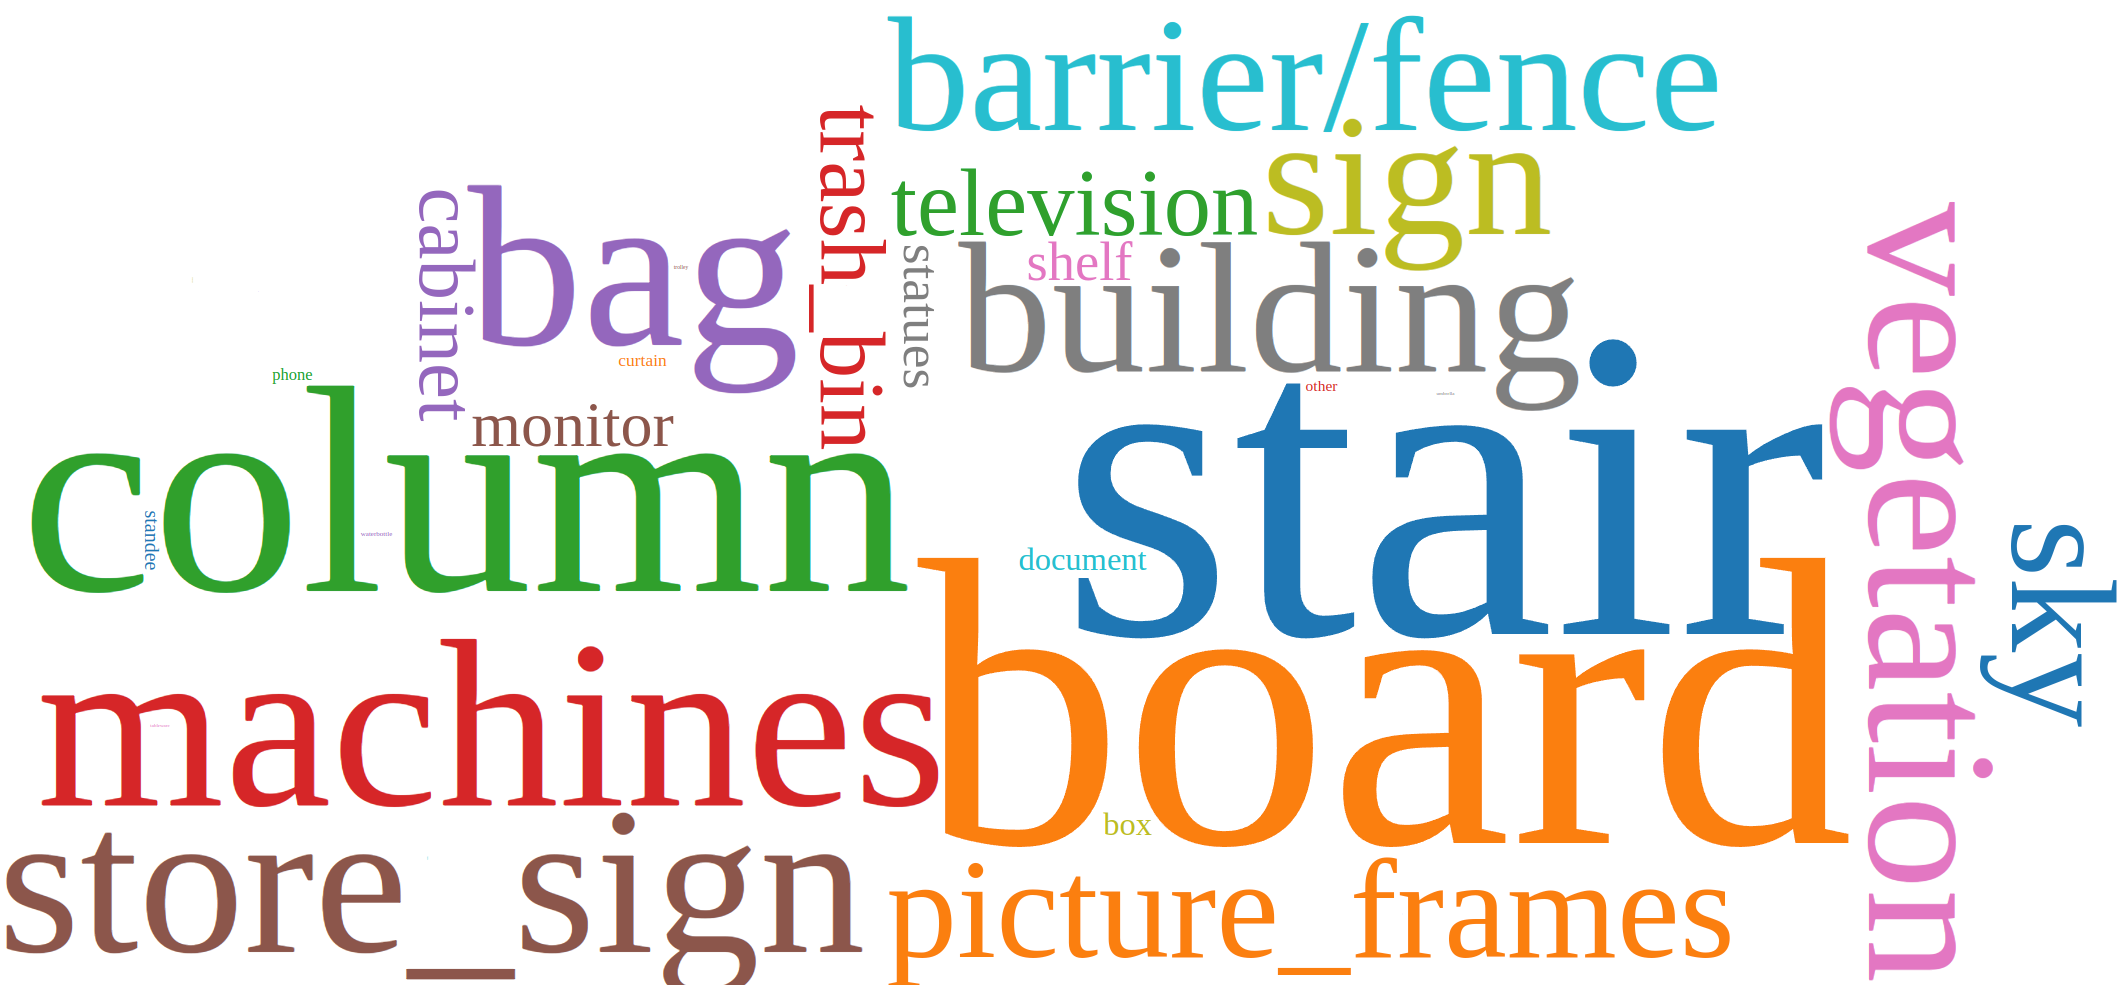}
%     \caption{Word cloud of the most frequent classes seen through glass in JRDB-PanoTrack, with the size of the word proportional to the frequency of the class.}
%     \label{fig:behind_glass_wordcloud}
%     \vspace{-1em}
% \end{figure}
\noindent\textbf{Behind glass.} Traditional datasets often assume that a pixel only belongs to a single object. However, as shown in \cref{fig:stacked_images}, in real-world environments, objects behind glass or being hung on wall also can be seen and are important for human-robot interaction, robot navigation and decision. Therefore, JRDB-PanoTrack provides annotations for such objects. \cref{fig:behind_glass_wordcloud} presents a word cloud of classes predominantly viewed through glass in JRDB-PanoTrack, emphasizing the prevalence of objects like \textit{board, stair, bag, machines,} and \textit{sign}.

\begin{figure*}[!ht]
    \centering
    \includegraphics[width=\linewidth]{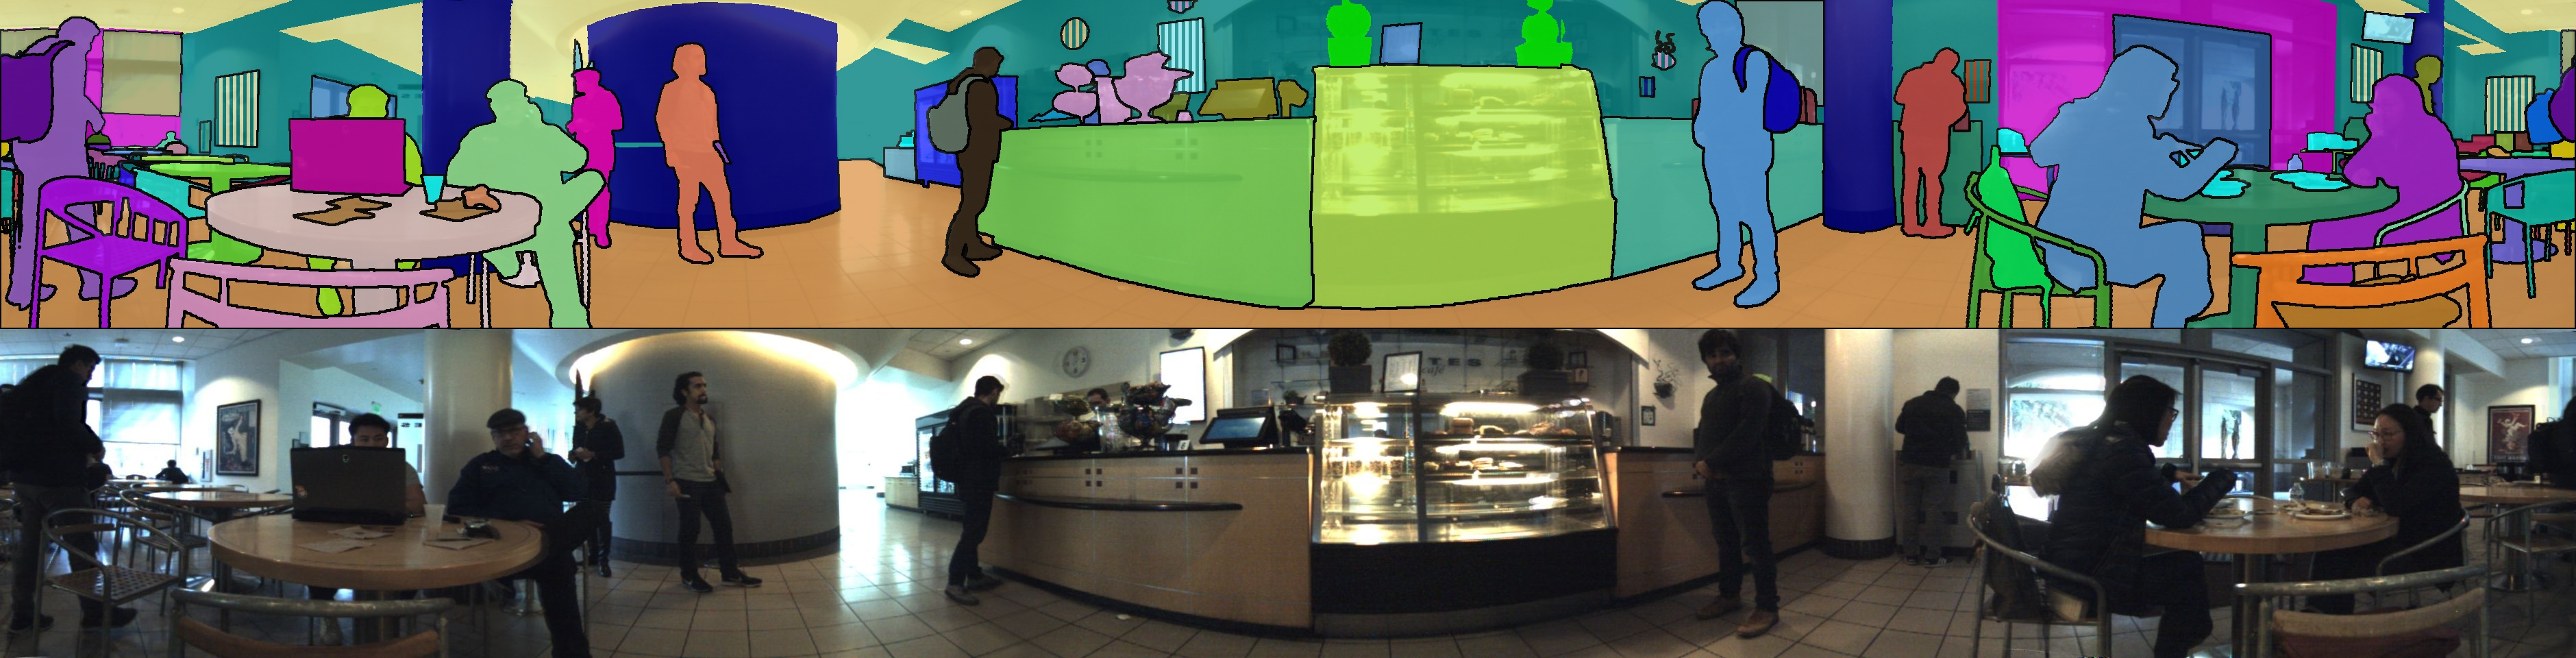}
    \includegraphics[width=\linewidth]{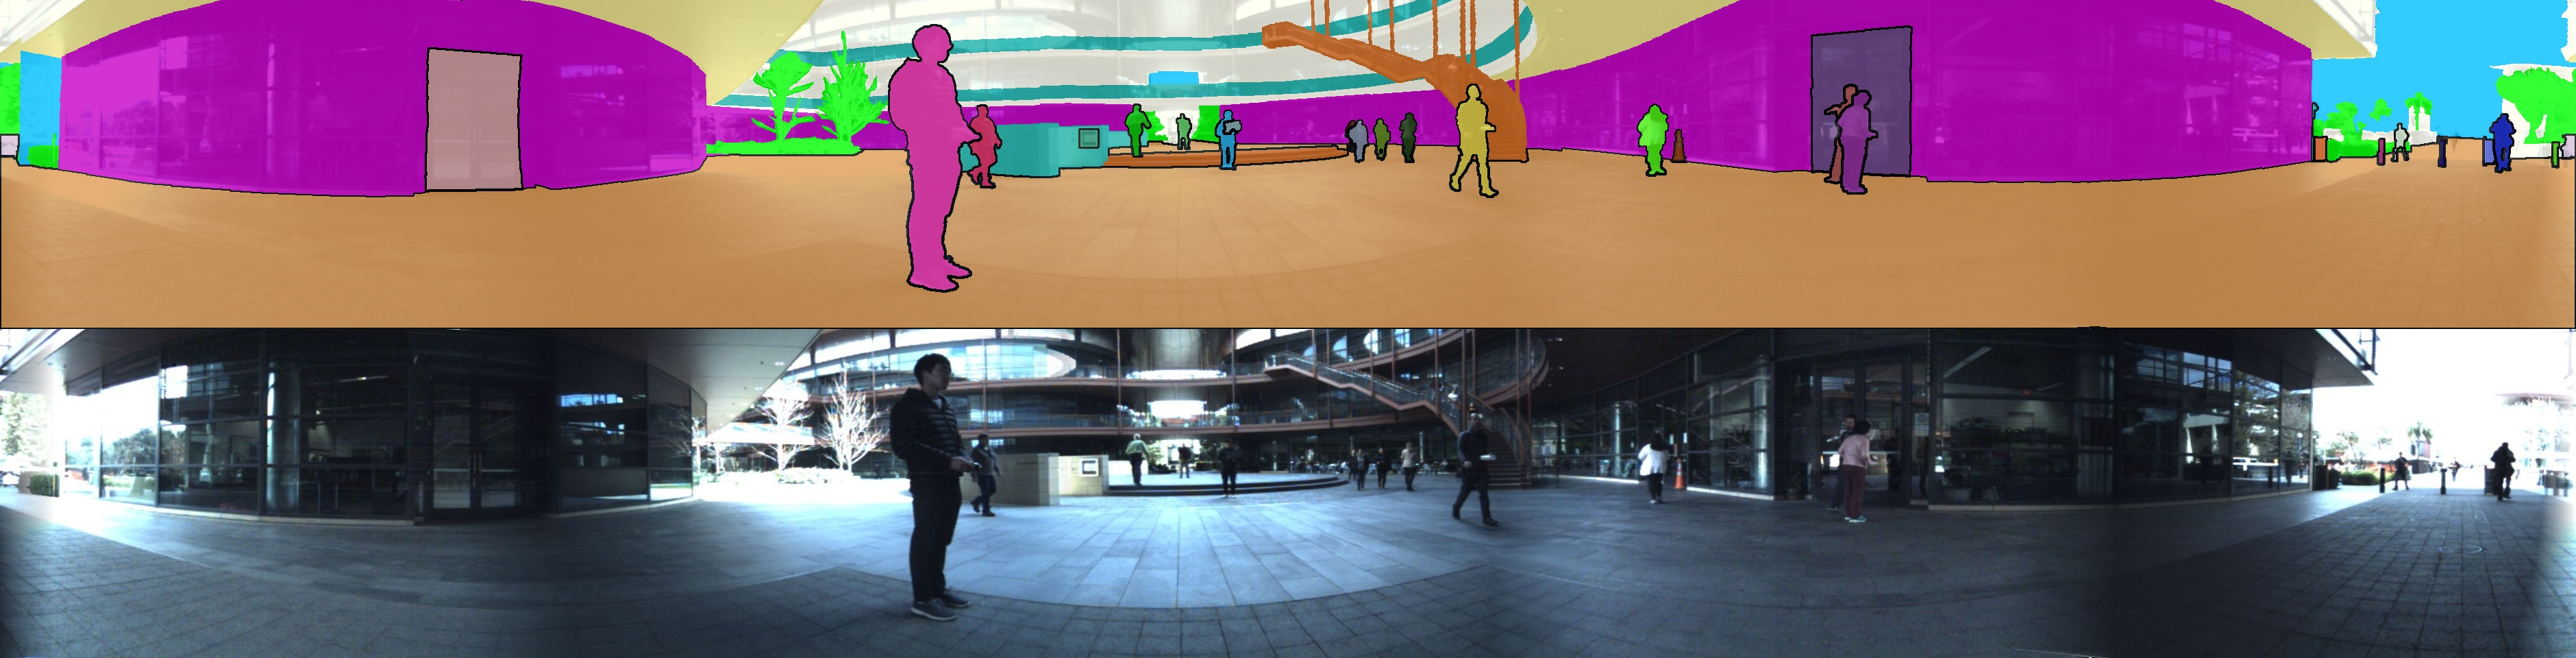}
    \includegraphics[width=\linewidth]{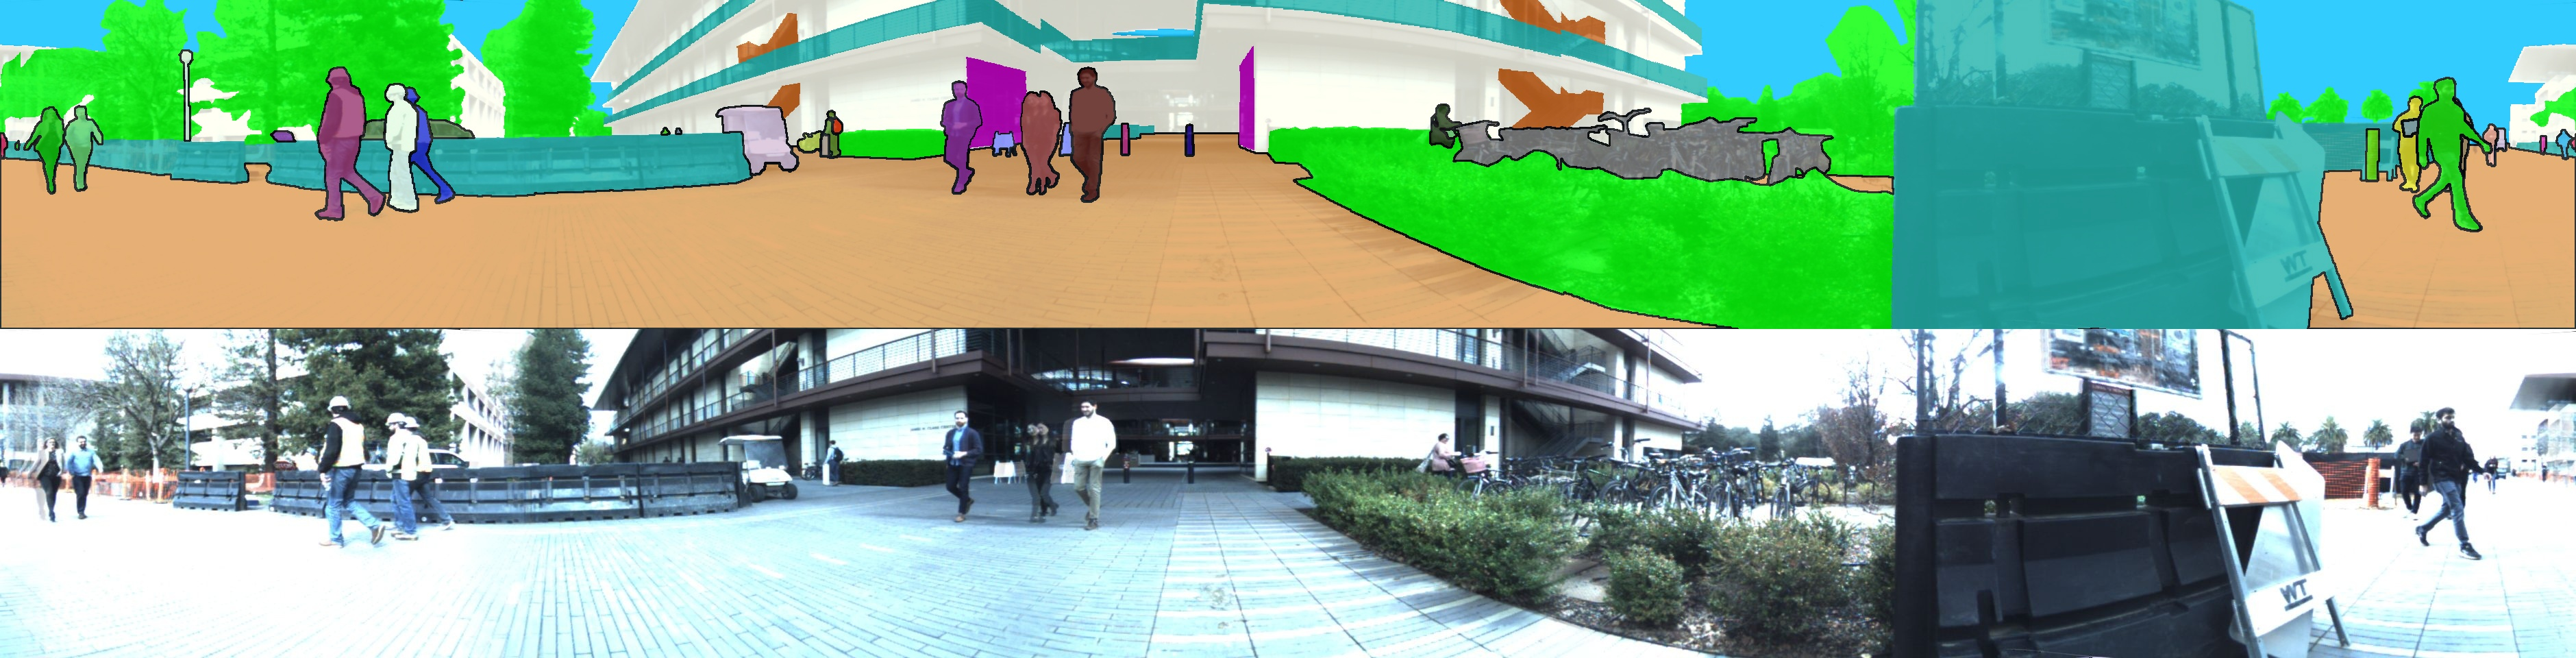}
    \includegraphics[width=\linewidth]{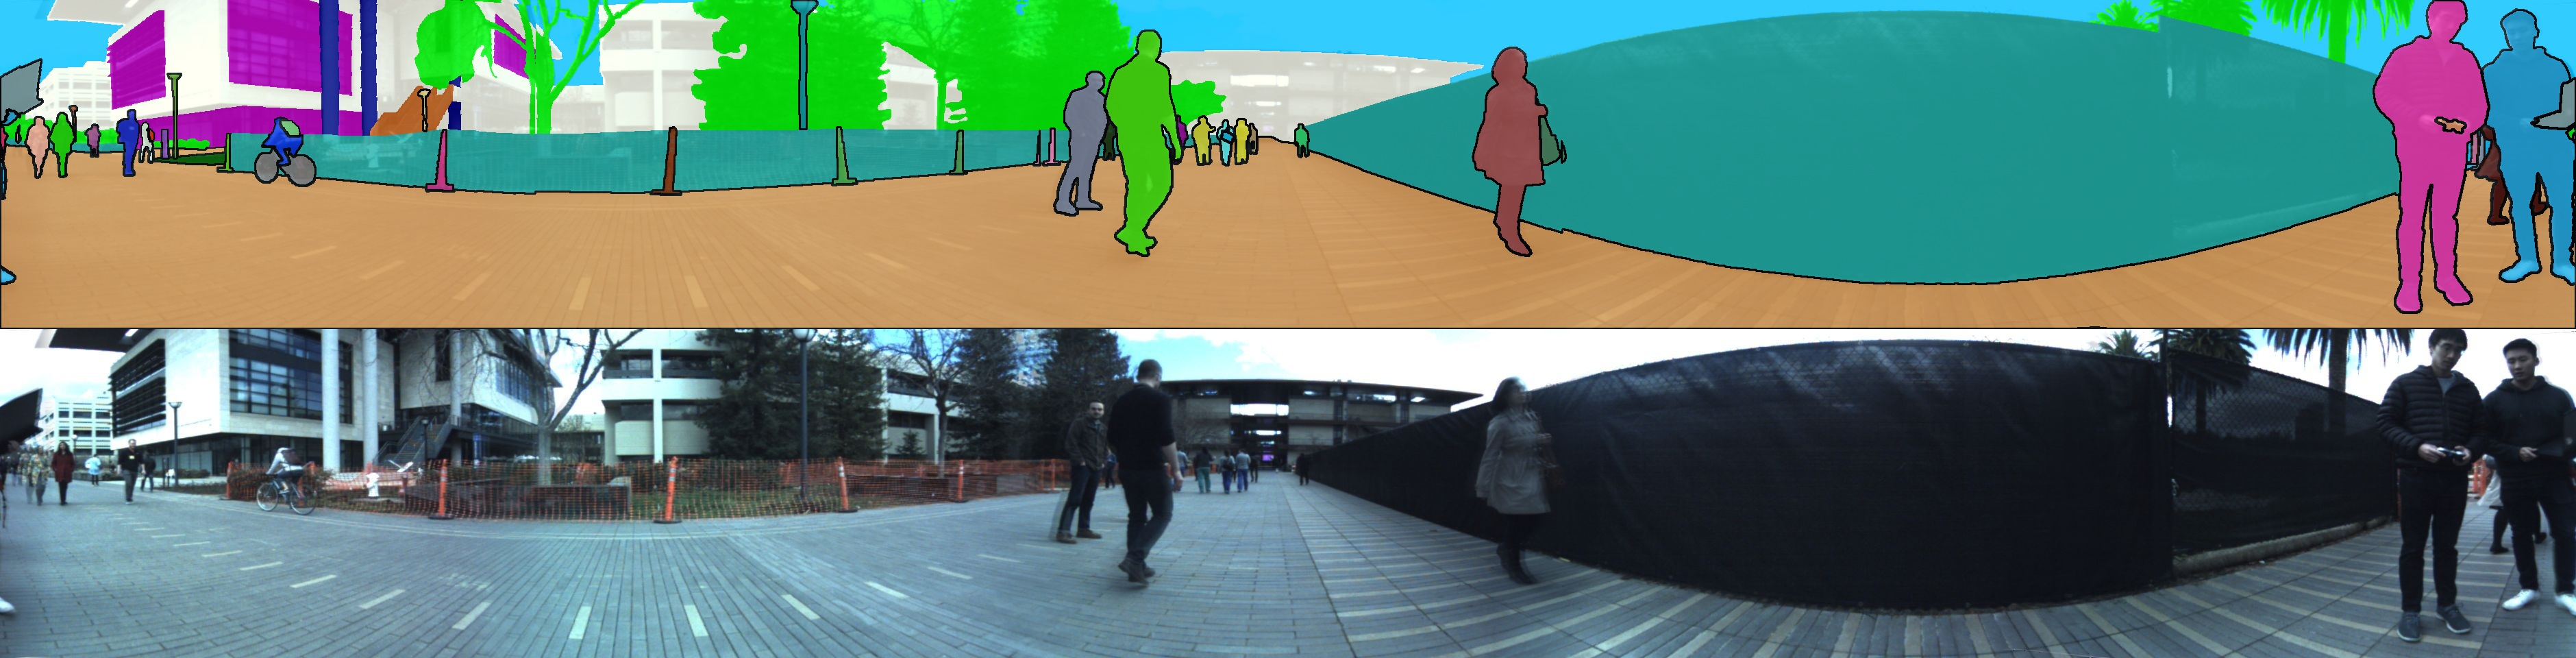}
    \includegraphics[width=\linewidth]{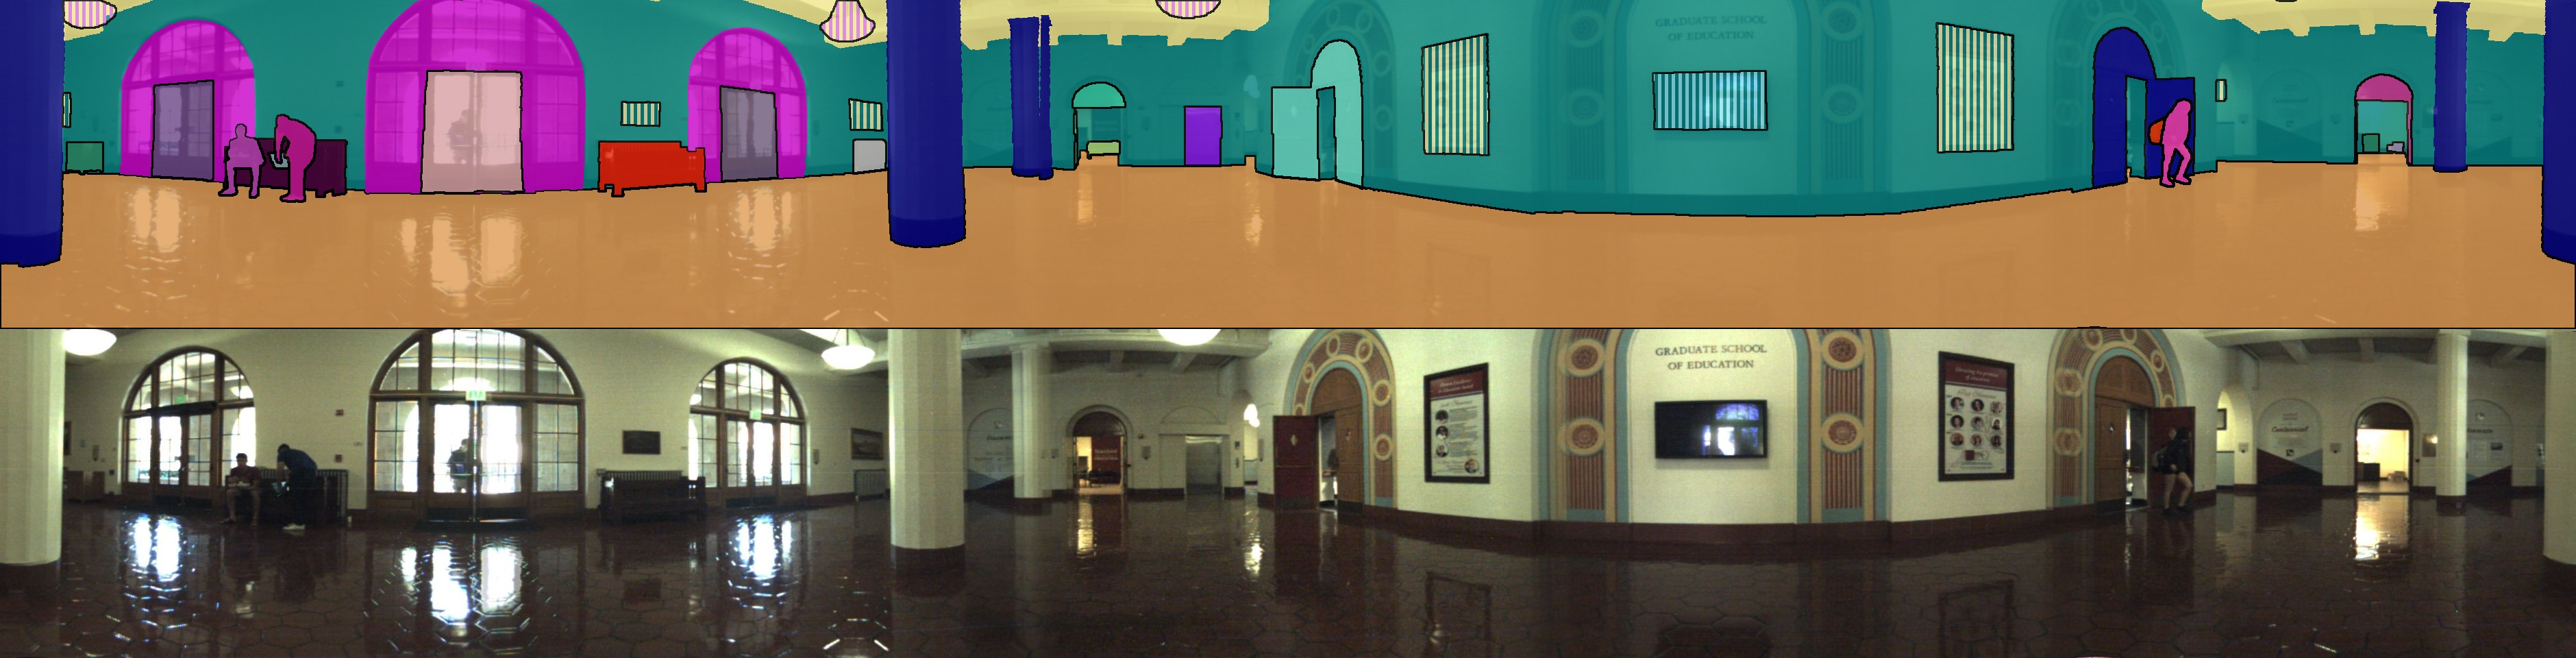}
\end{figure*}

\begin{figure*}[!ht]
    \centering
    \includegraphics[width=\linewidth]{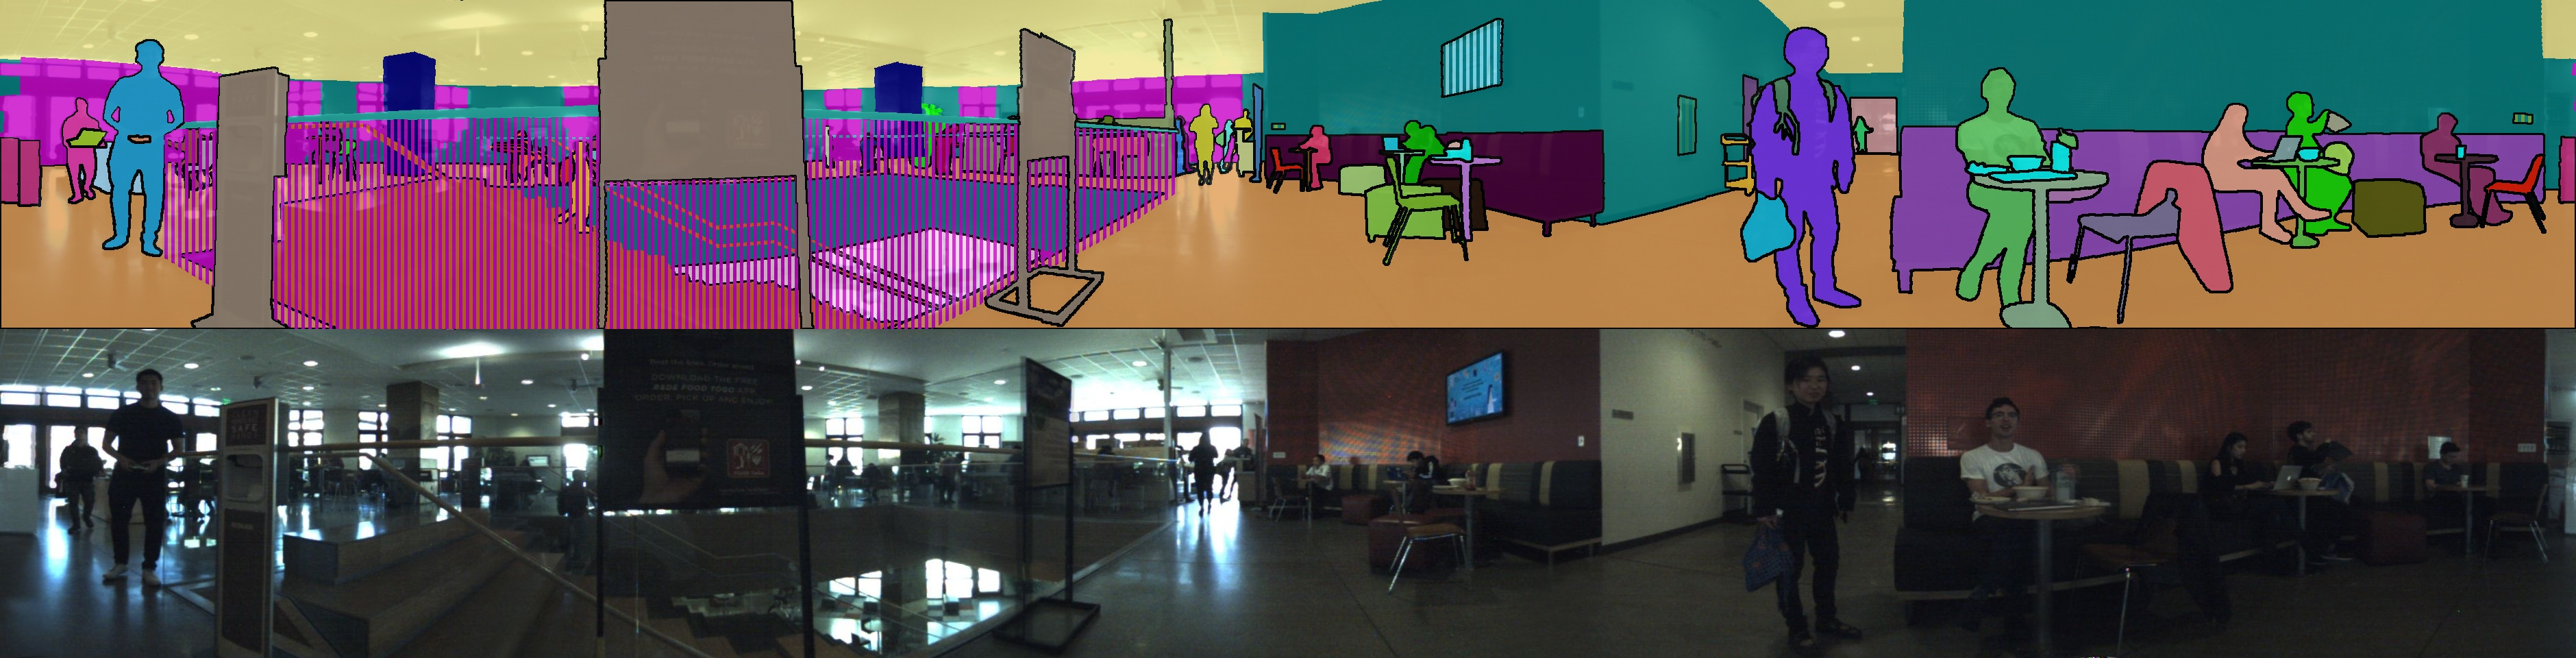}
    \includegraphics[width=\linewidth]{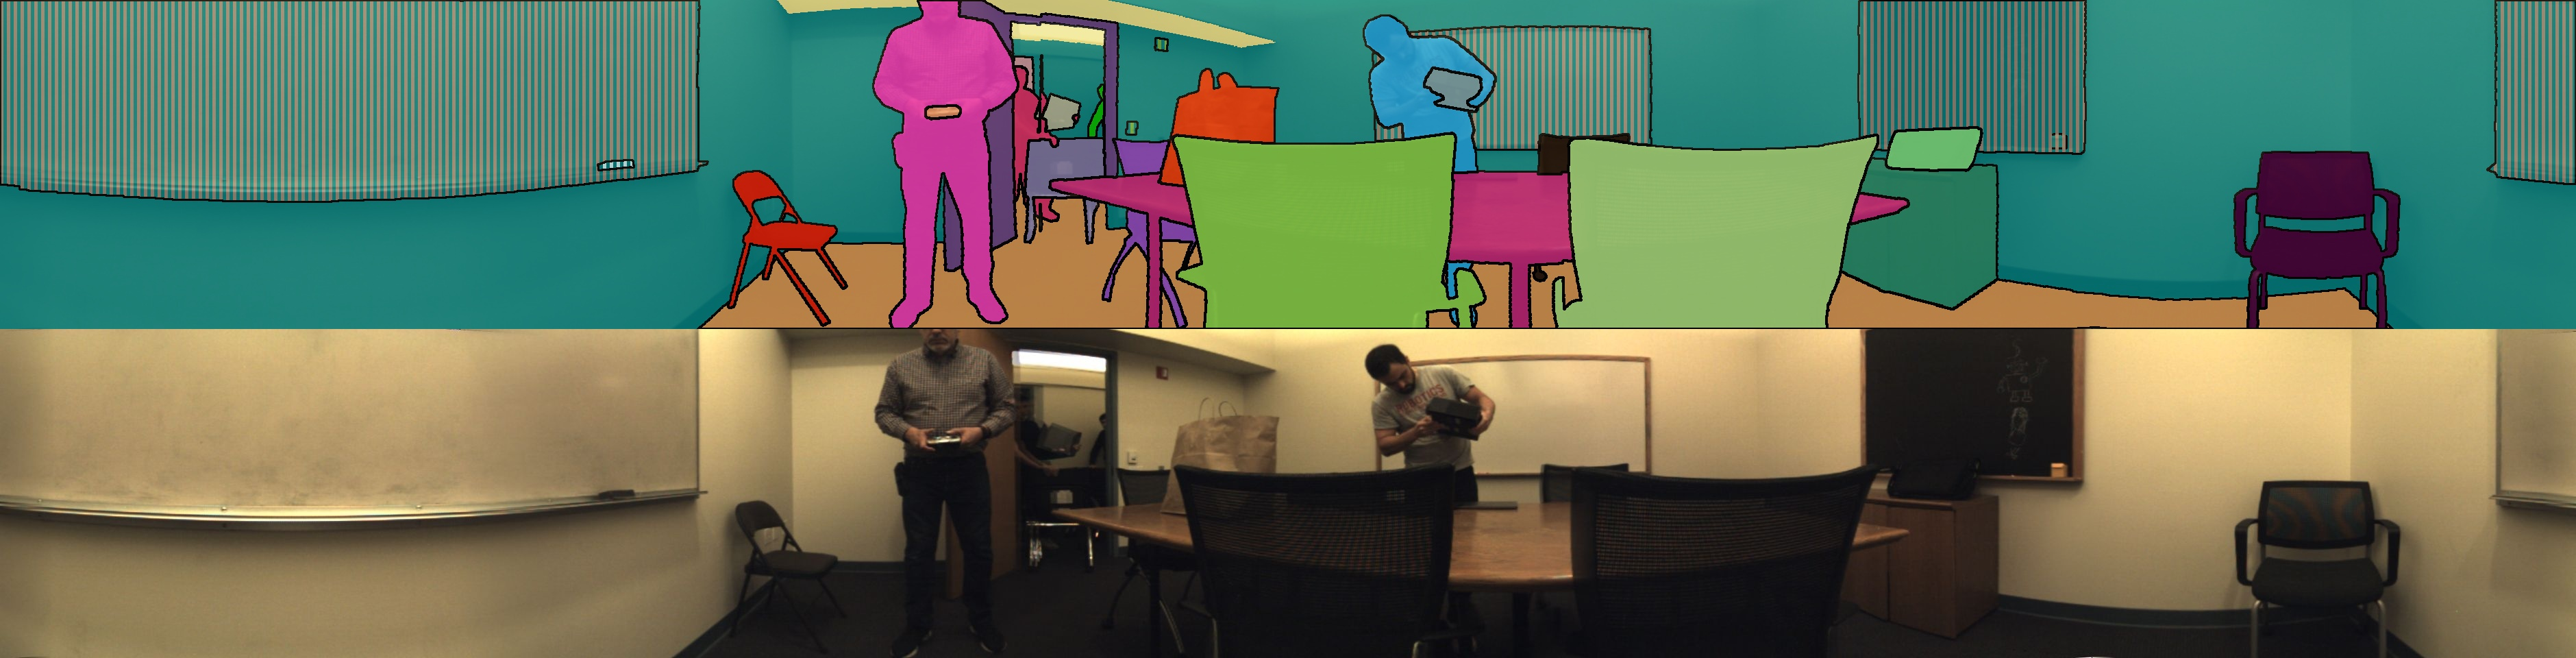}
    \includegraphics[width=\linewidth]{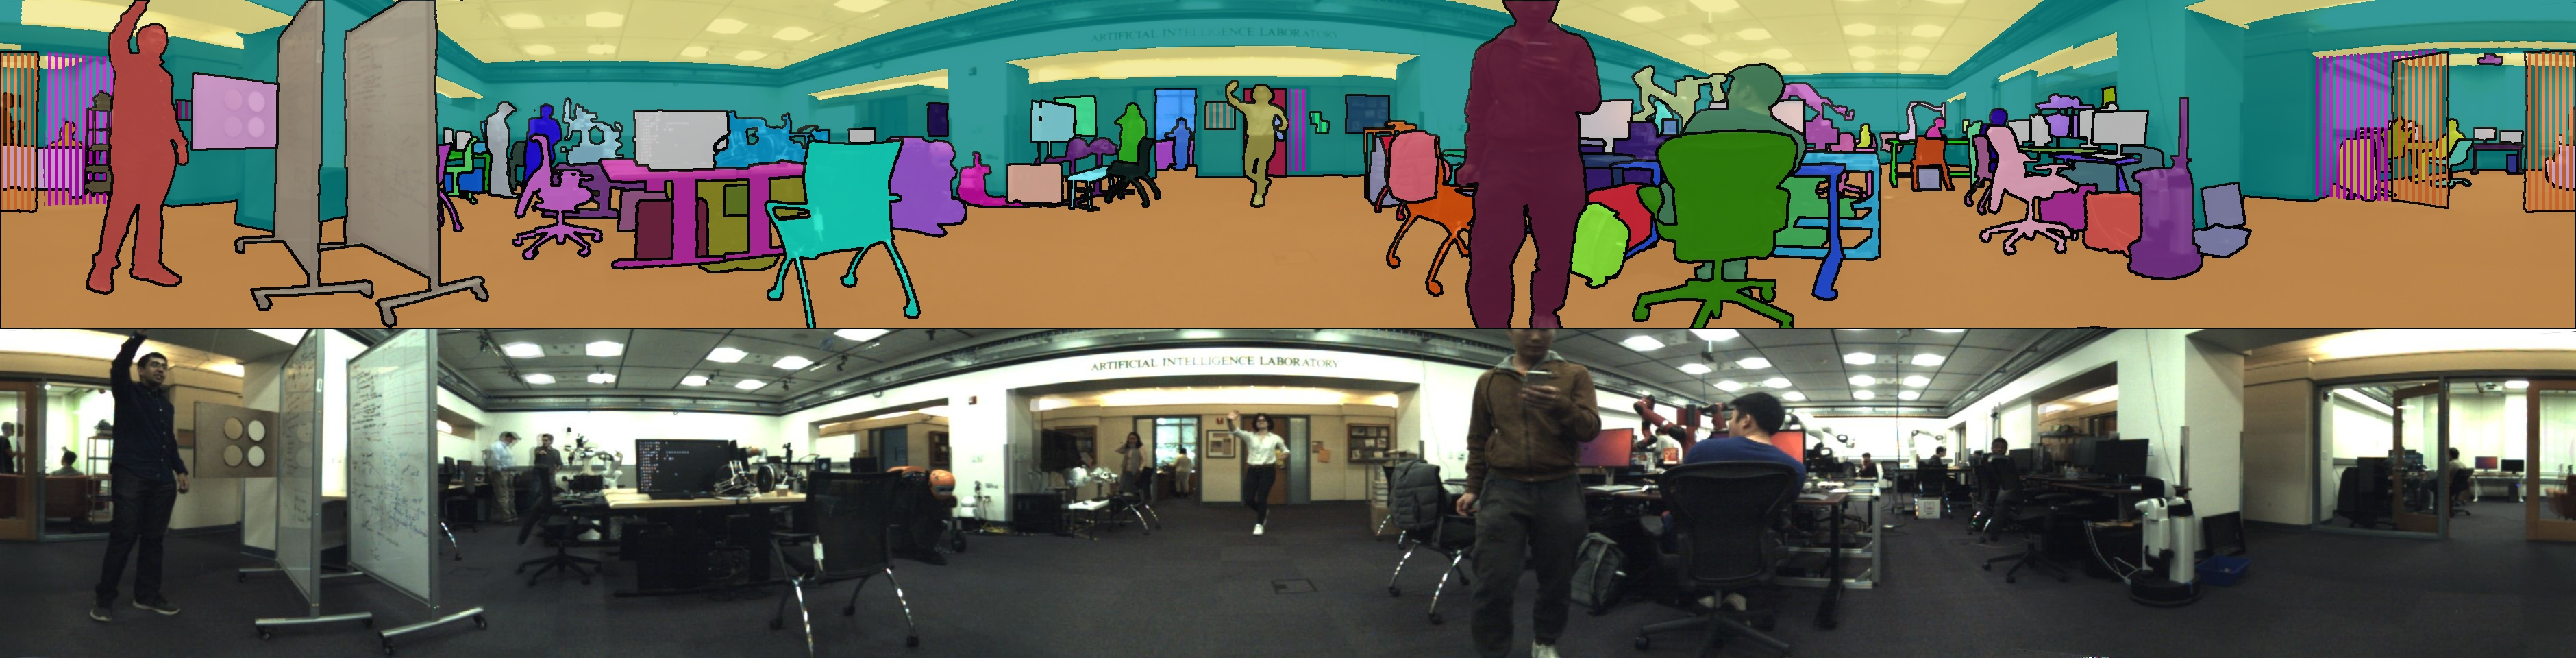}
    \includegraphics[width=\linewidth]{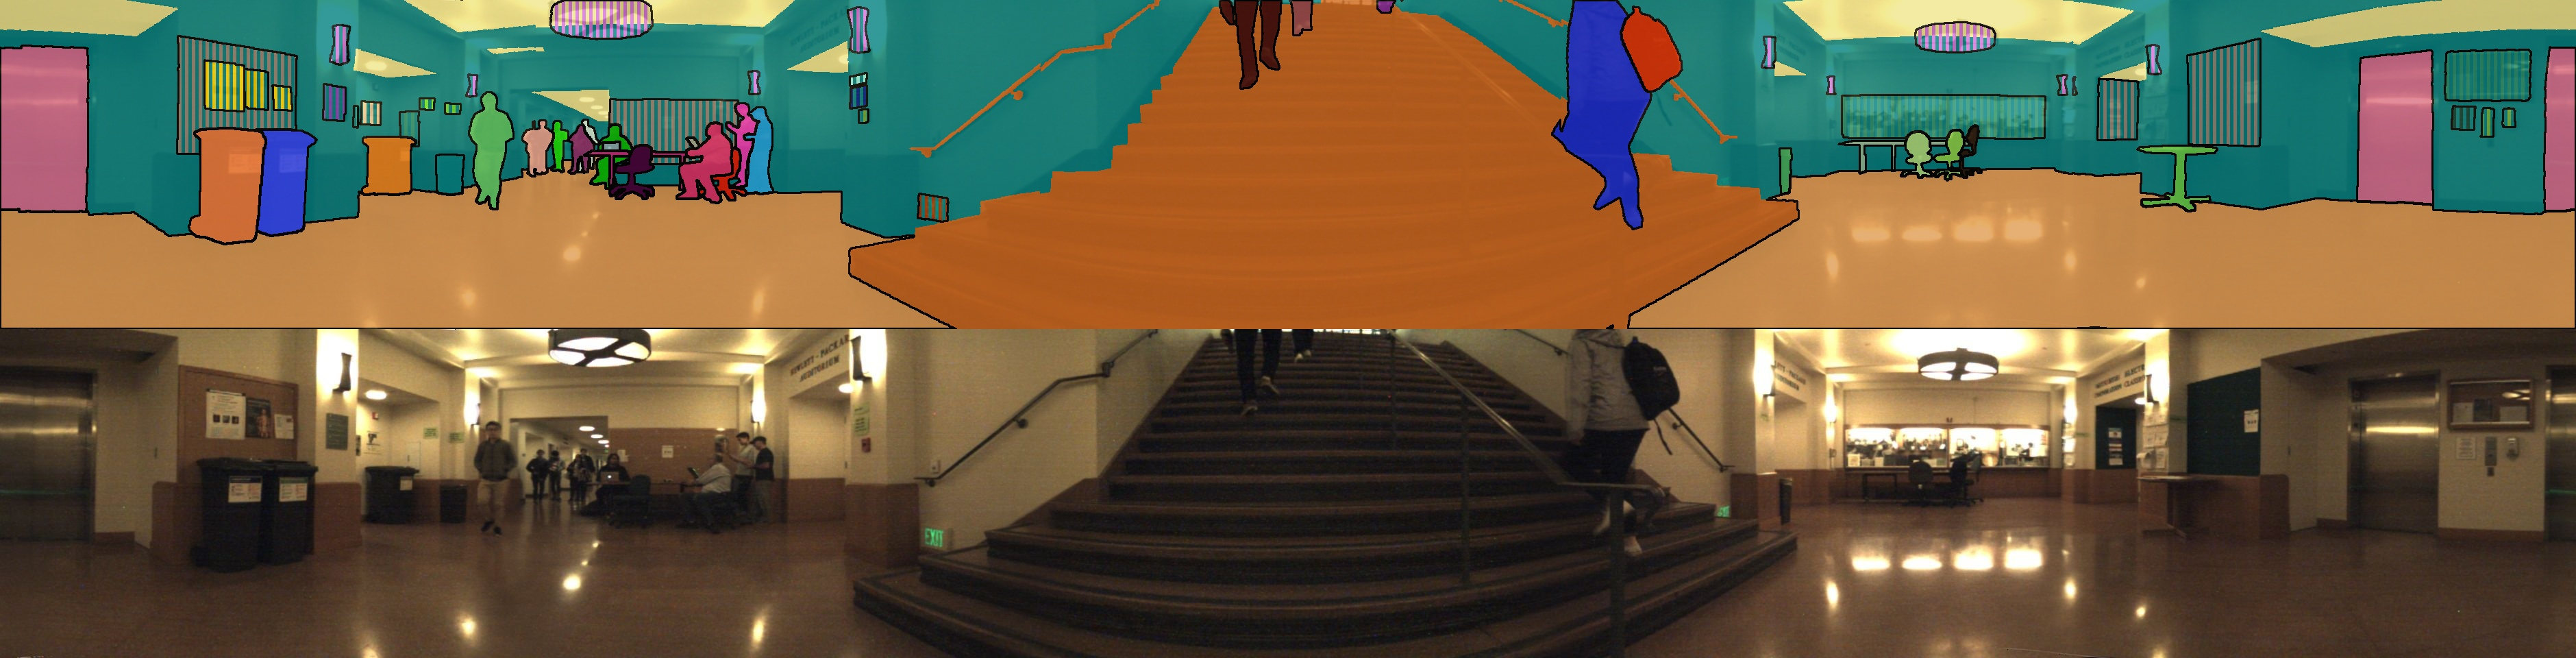}
    \includegraphics[width=\linewidth]{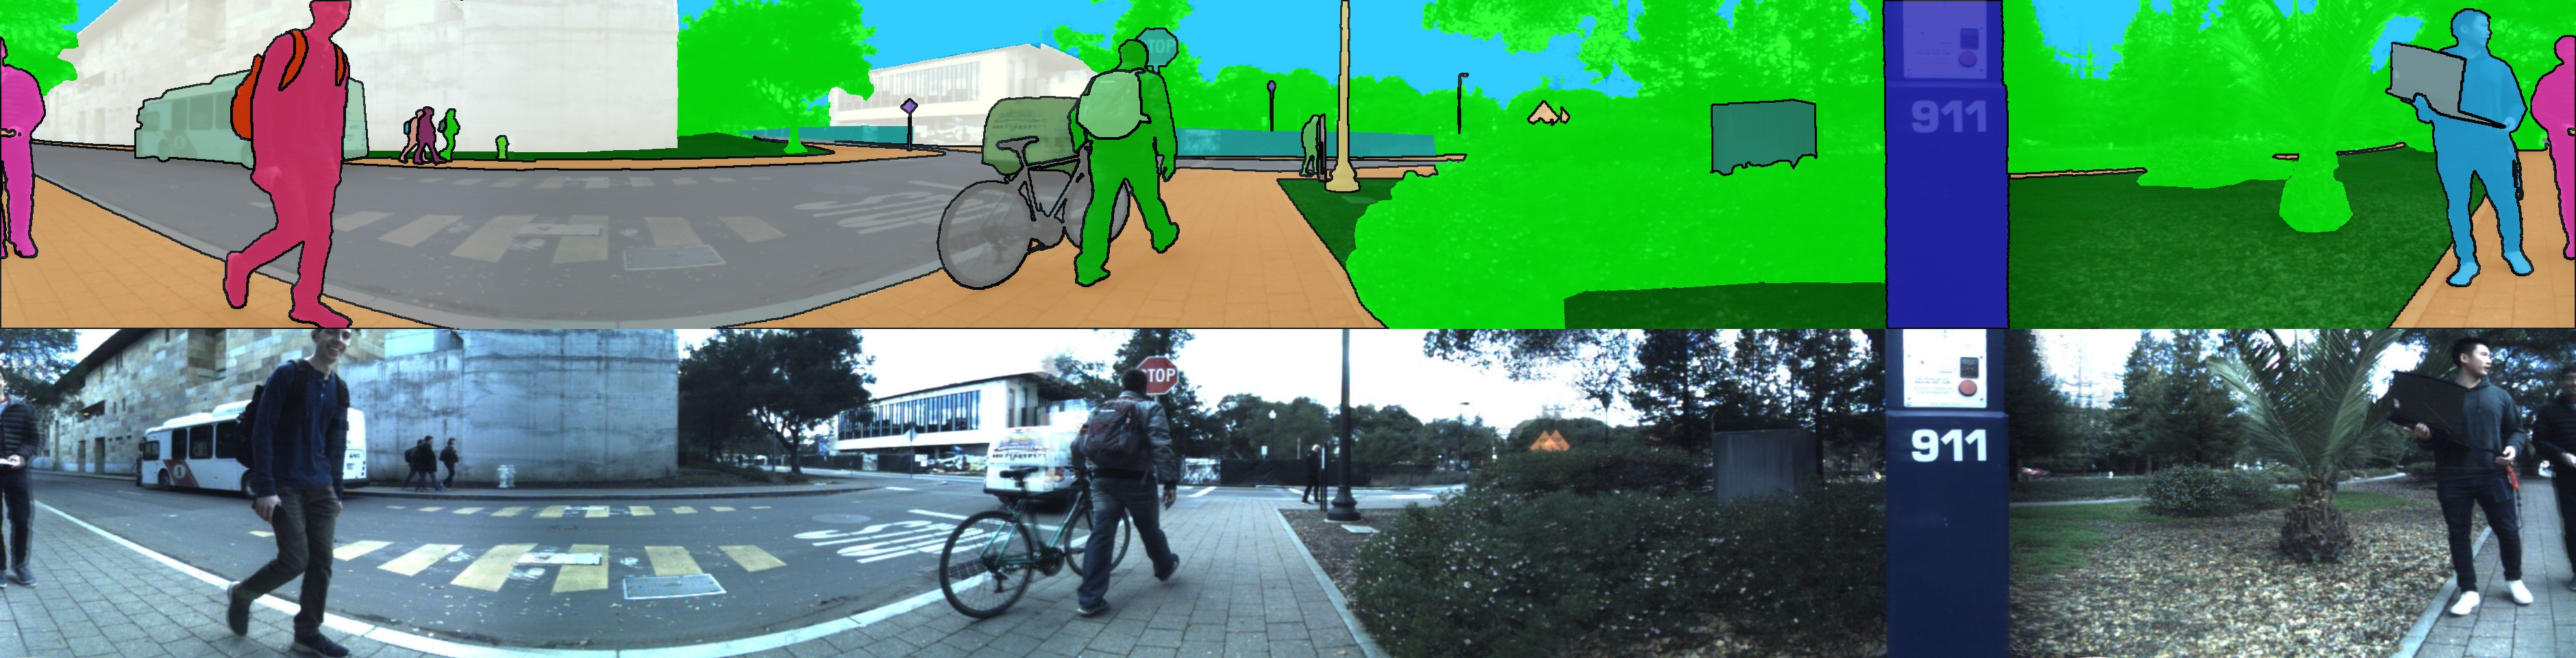}
\end{figure*}

\begin{figure*}[!ht]
    \centering
    \includegraphics[width=\linewidth]{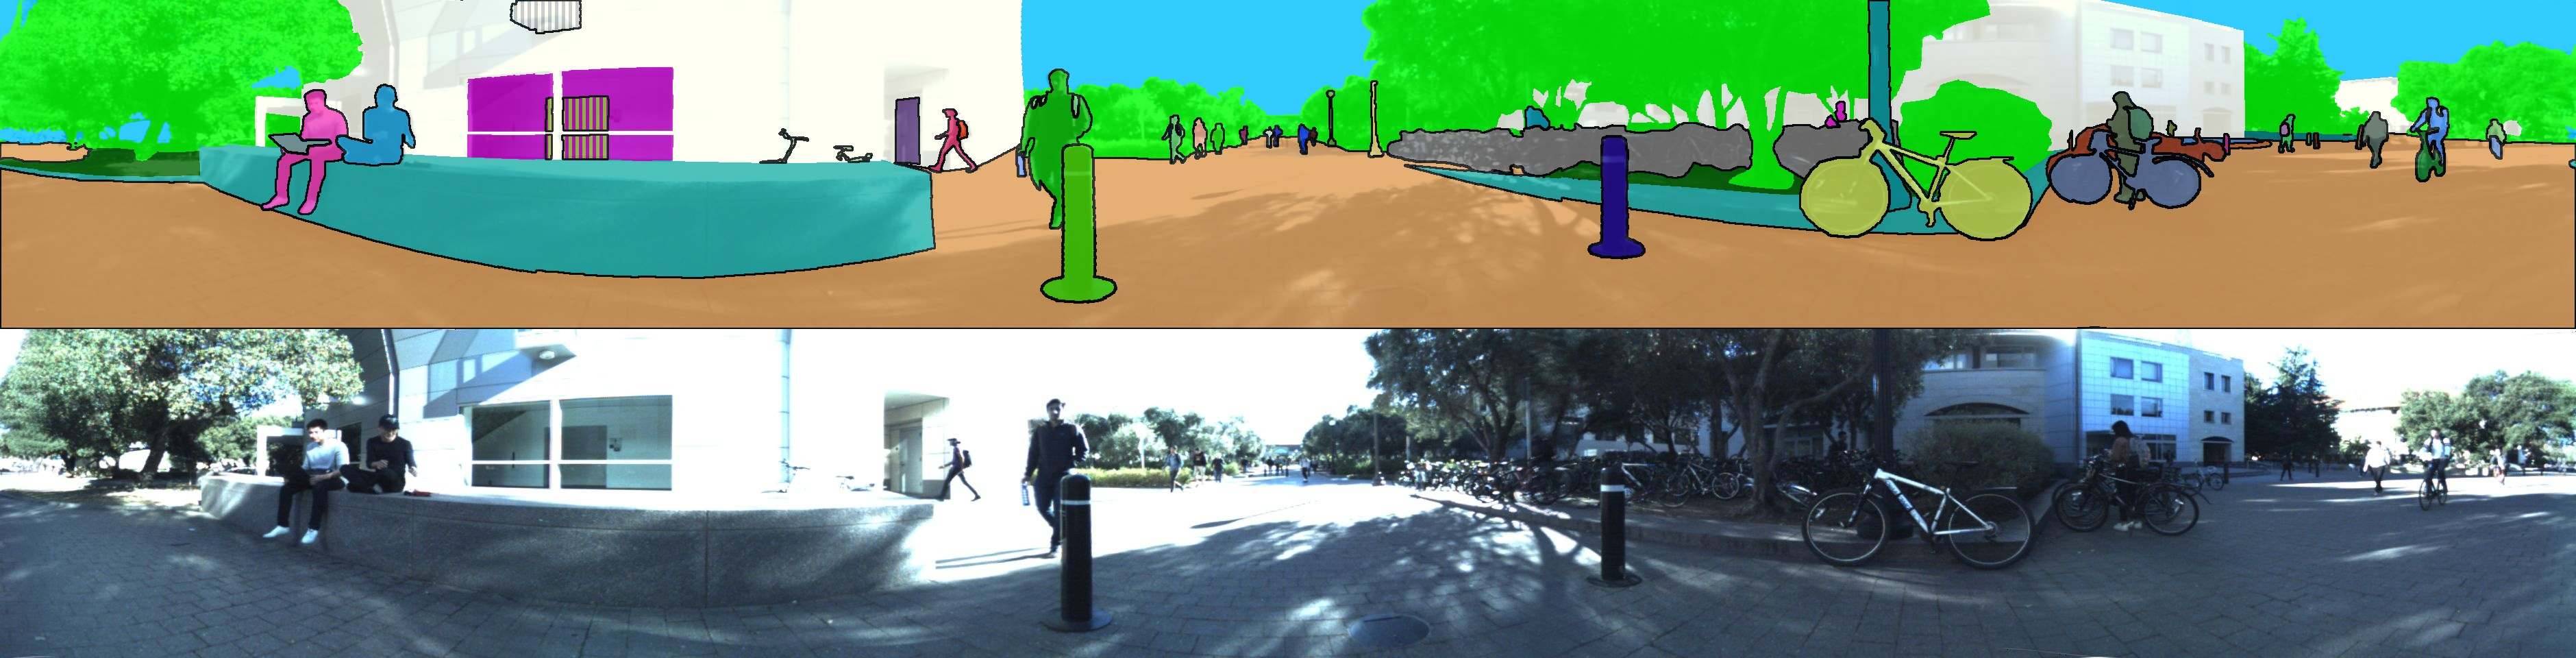}
    \includegraphics[width=\linewidth]{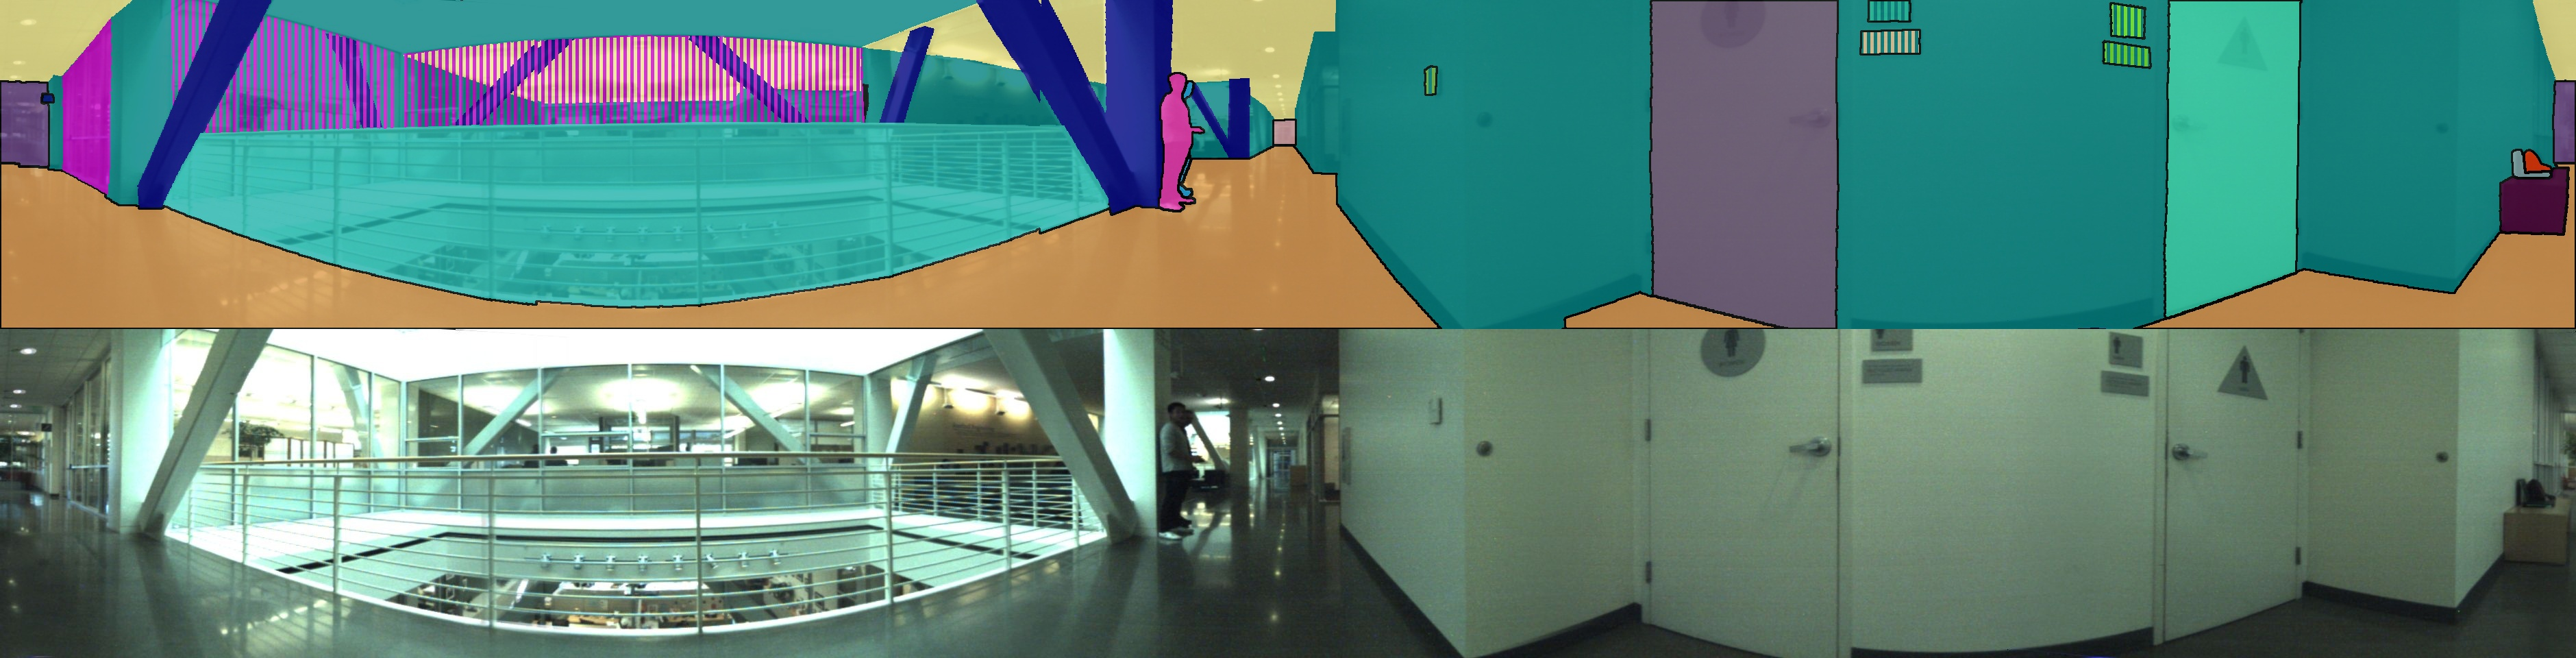}
    \includegraphics[width=\linewidth]{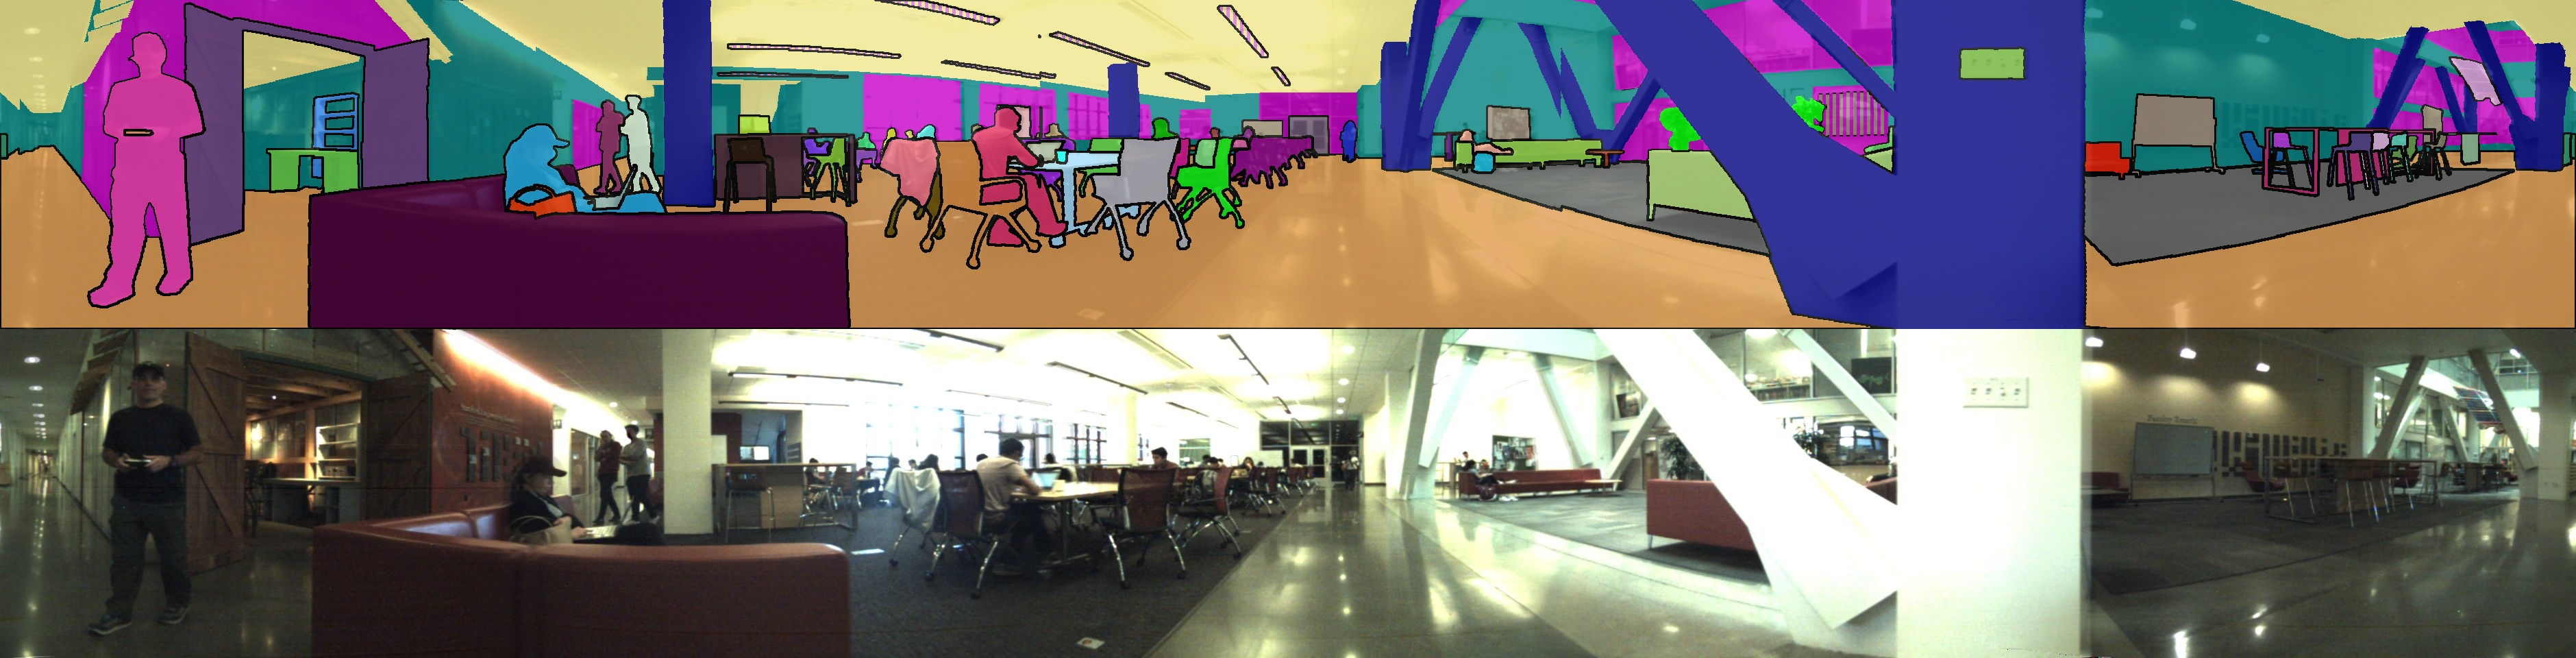}
    \includegraphics[width=\linewidth]{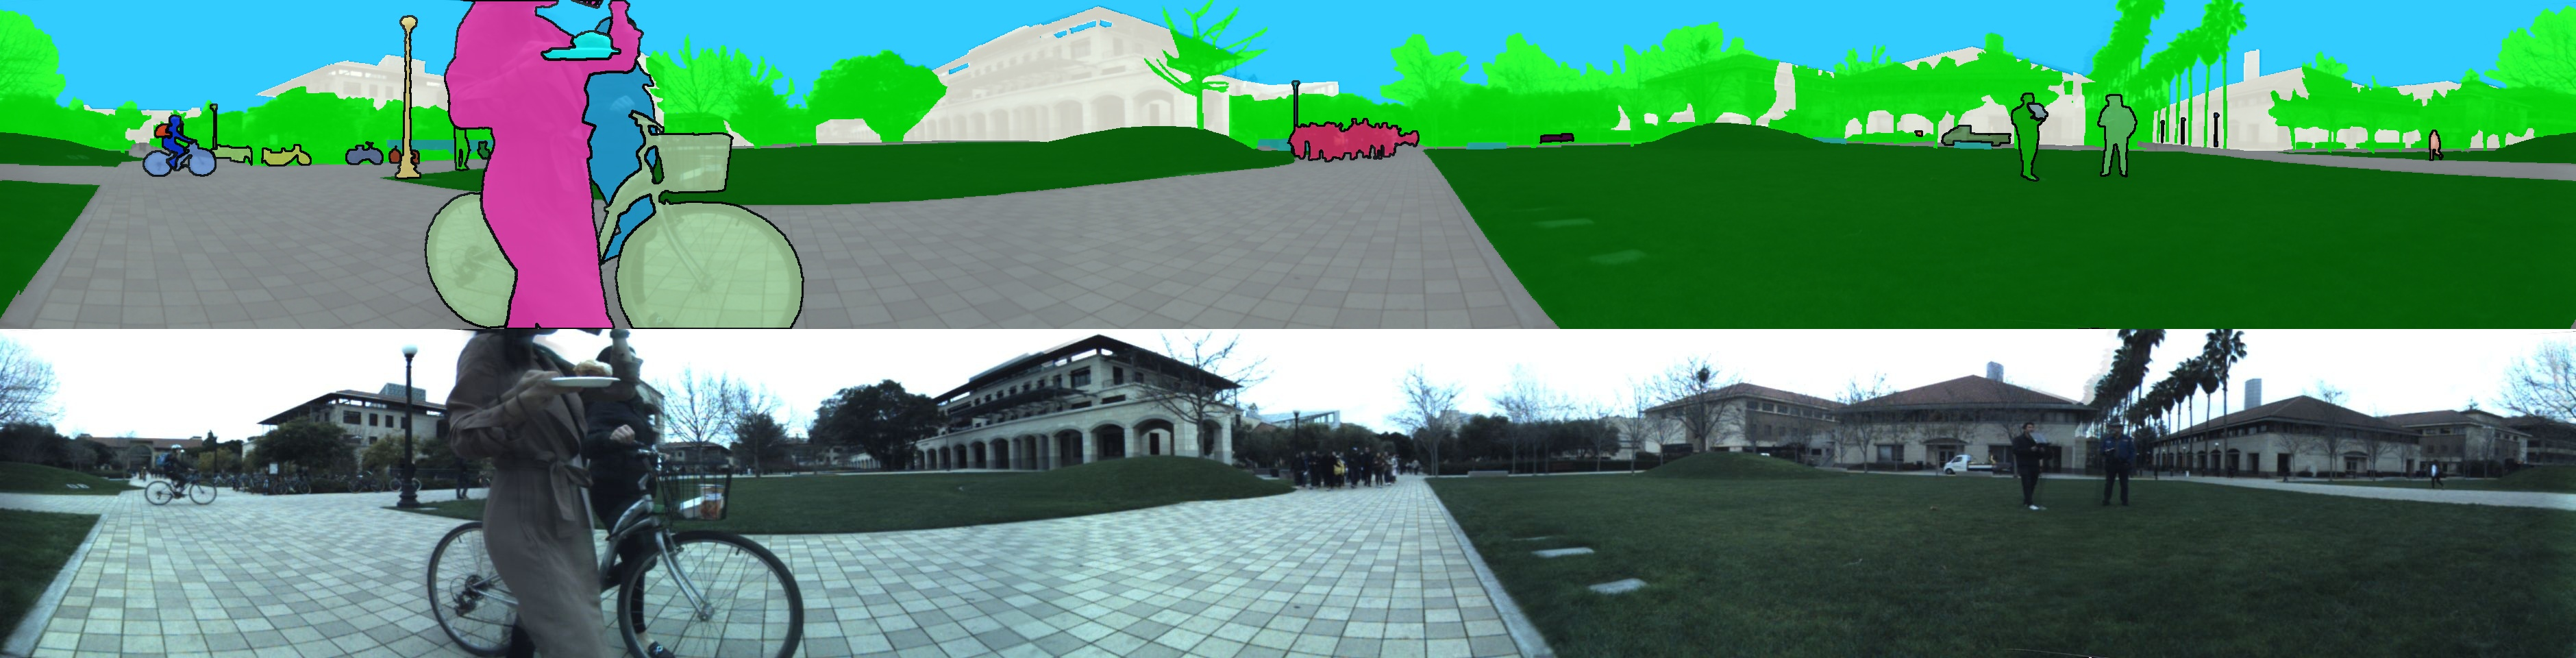}
    \includegraphics[width=\linewidth]{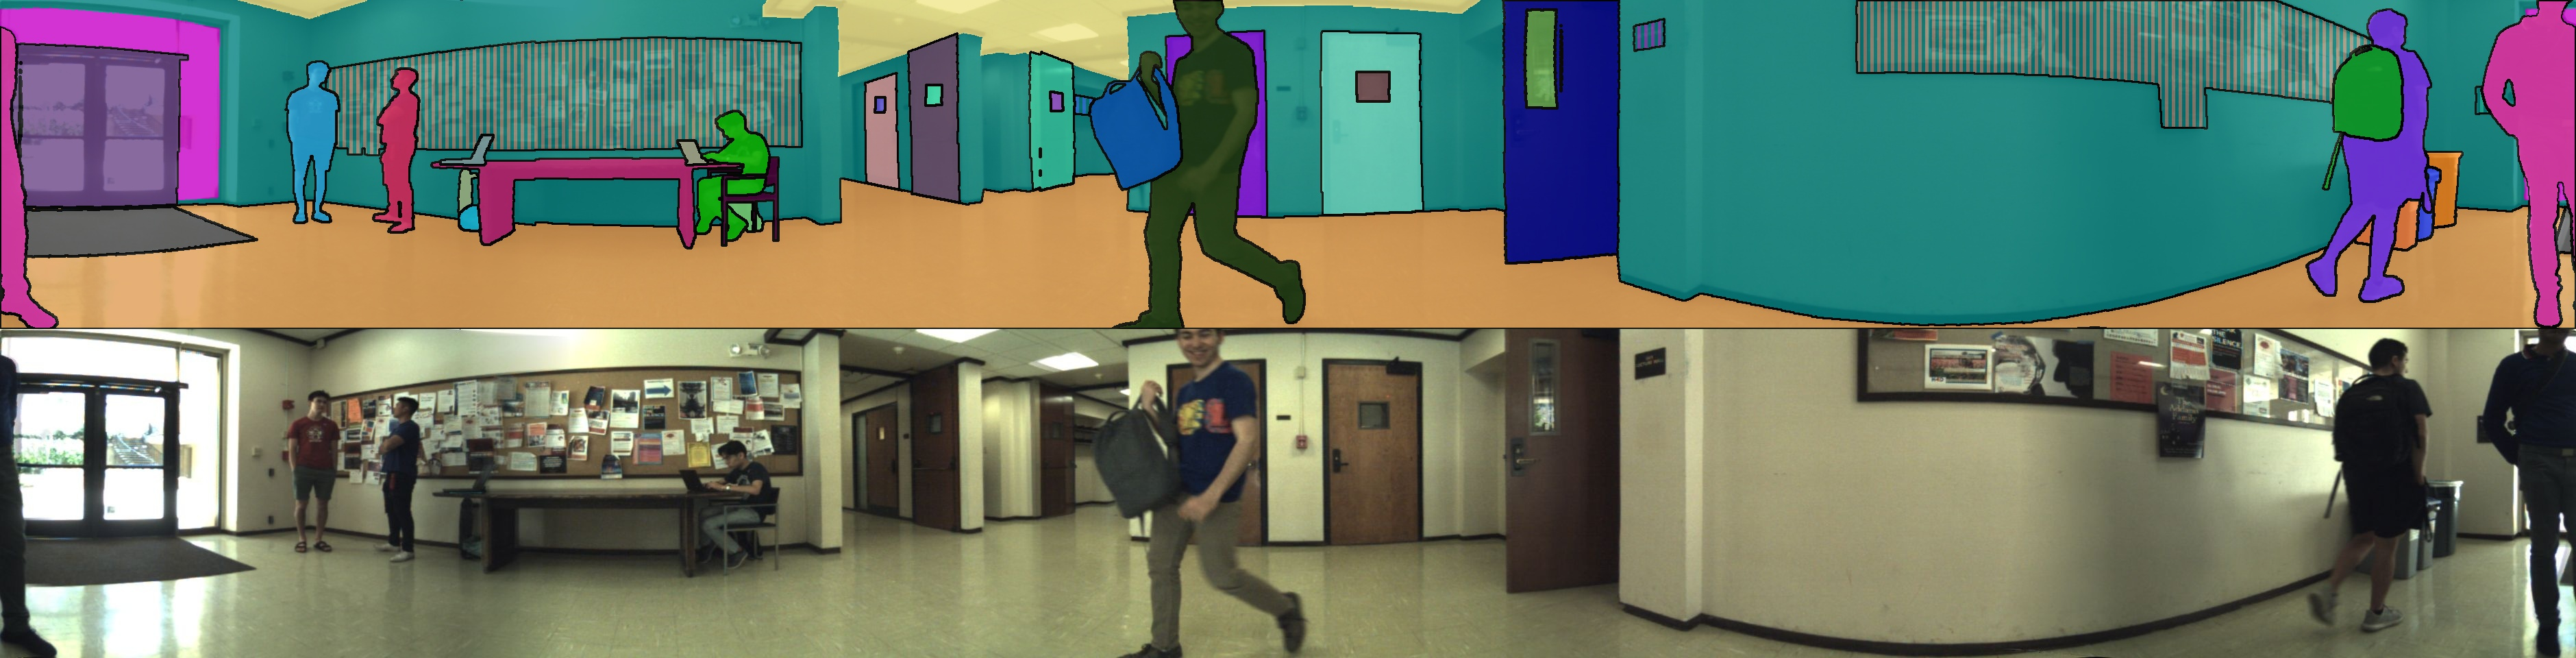}
\end{figure*}

\begin{figure*}[!ht]
    \centering
    \includegraphics[width=\linewidth]{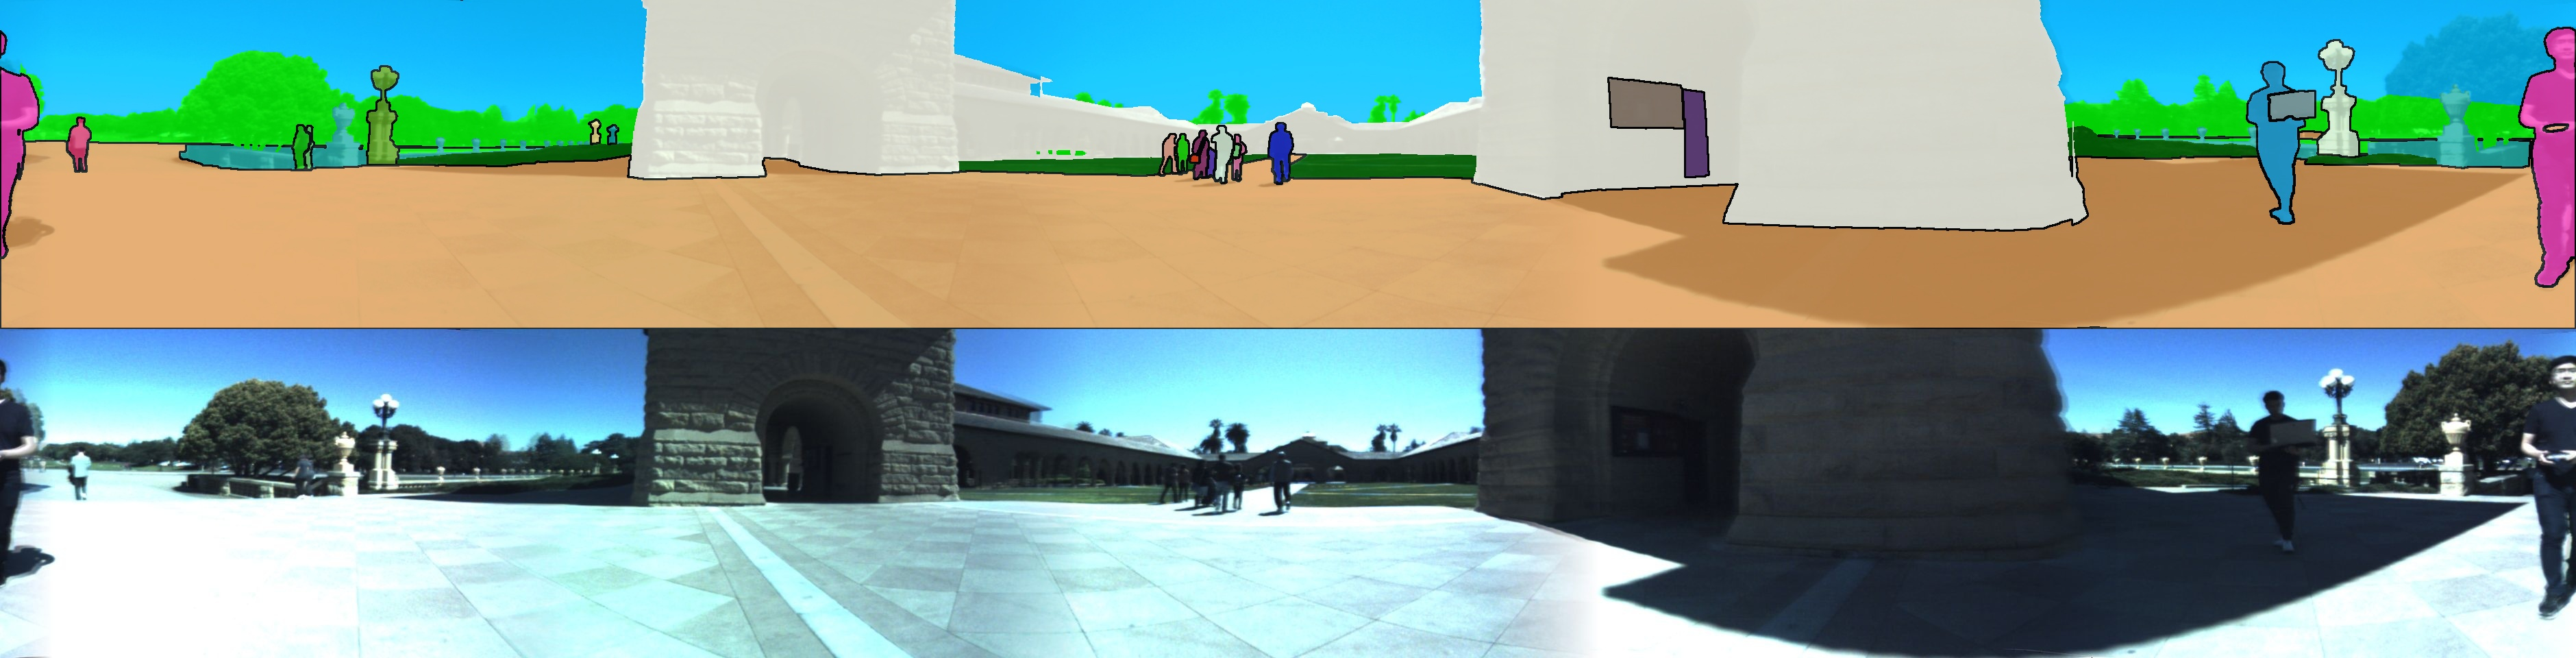}
    \includegraphics[width=\linewidth]{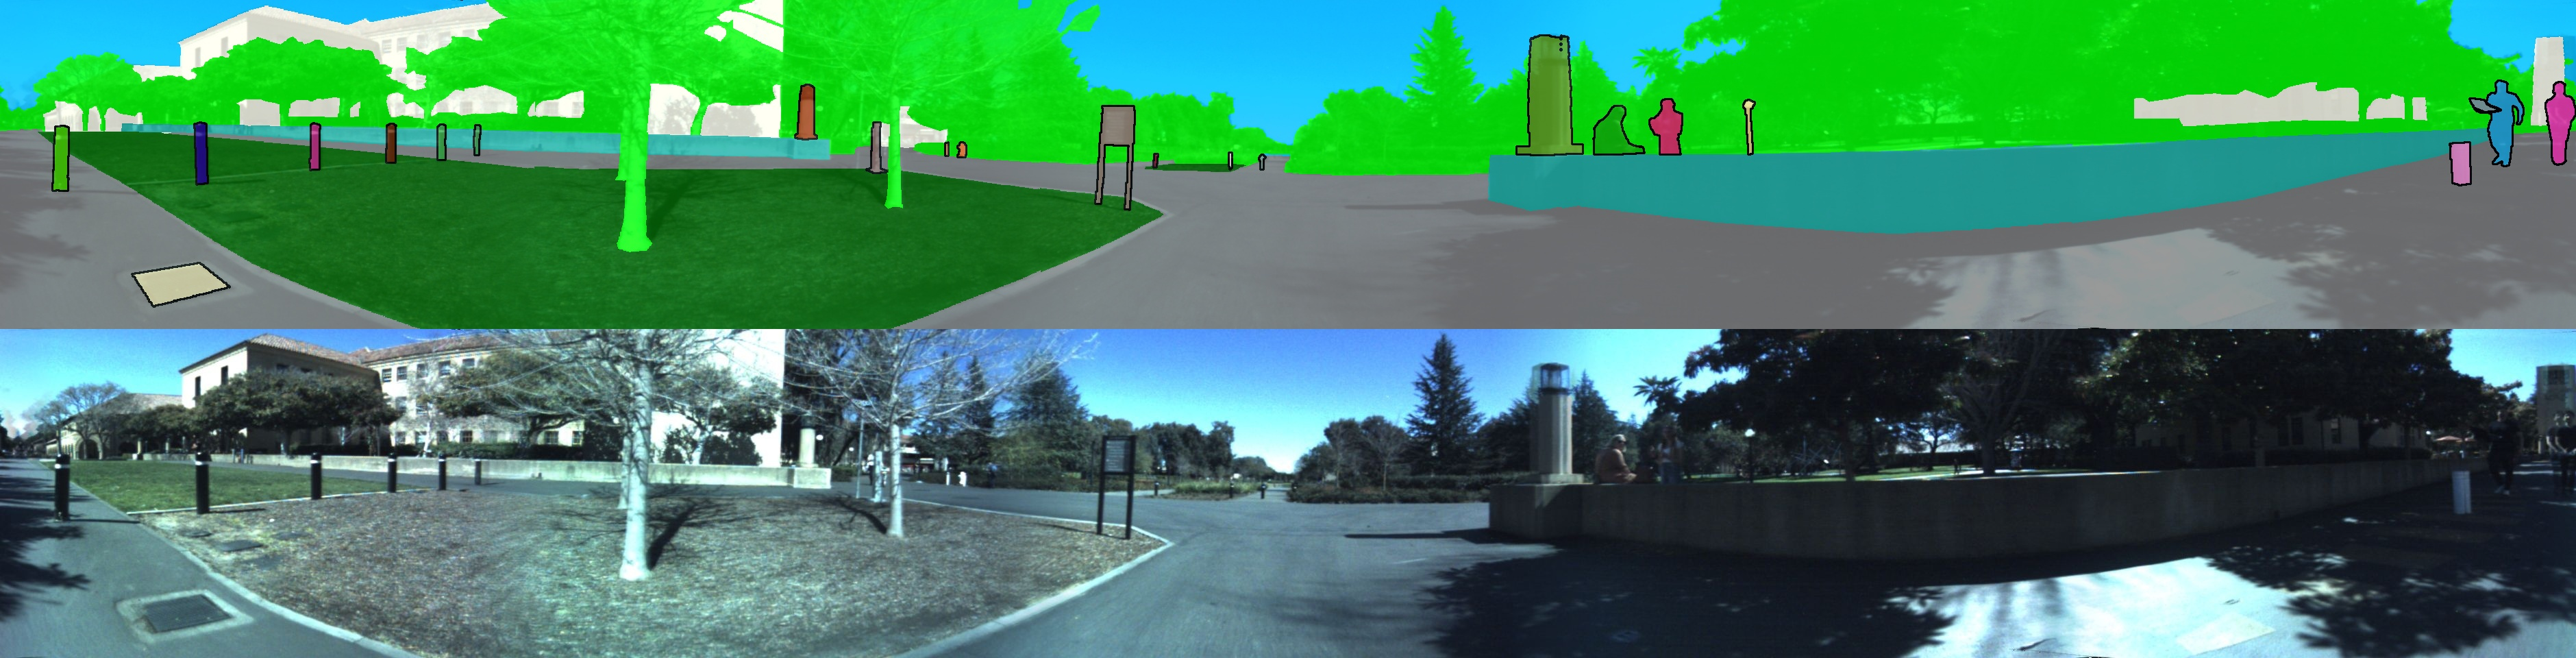}
    \includegraphics[width=\linewidth]{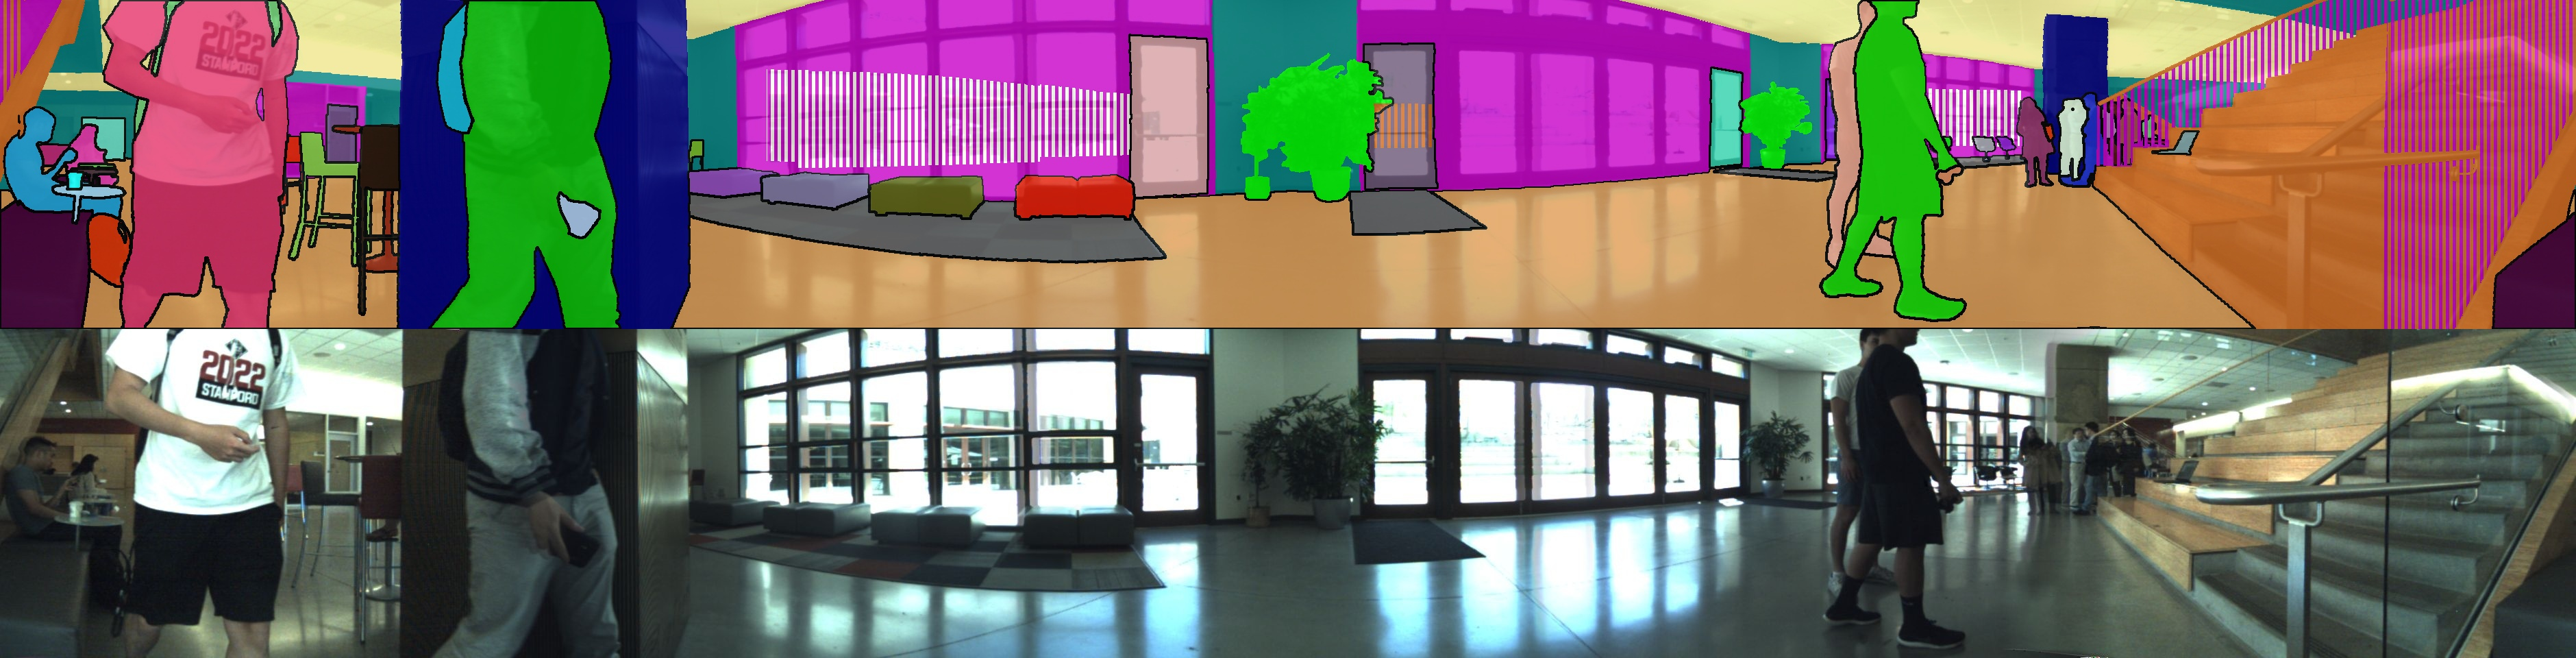}
    \includegraphics[width=\linewidth]{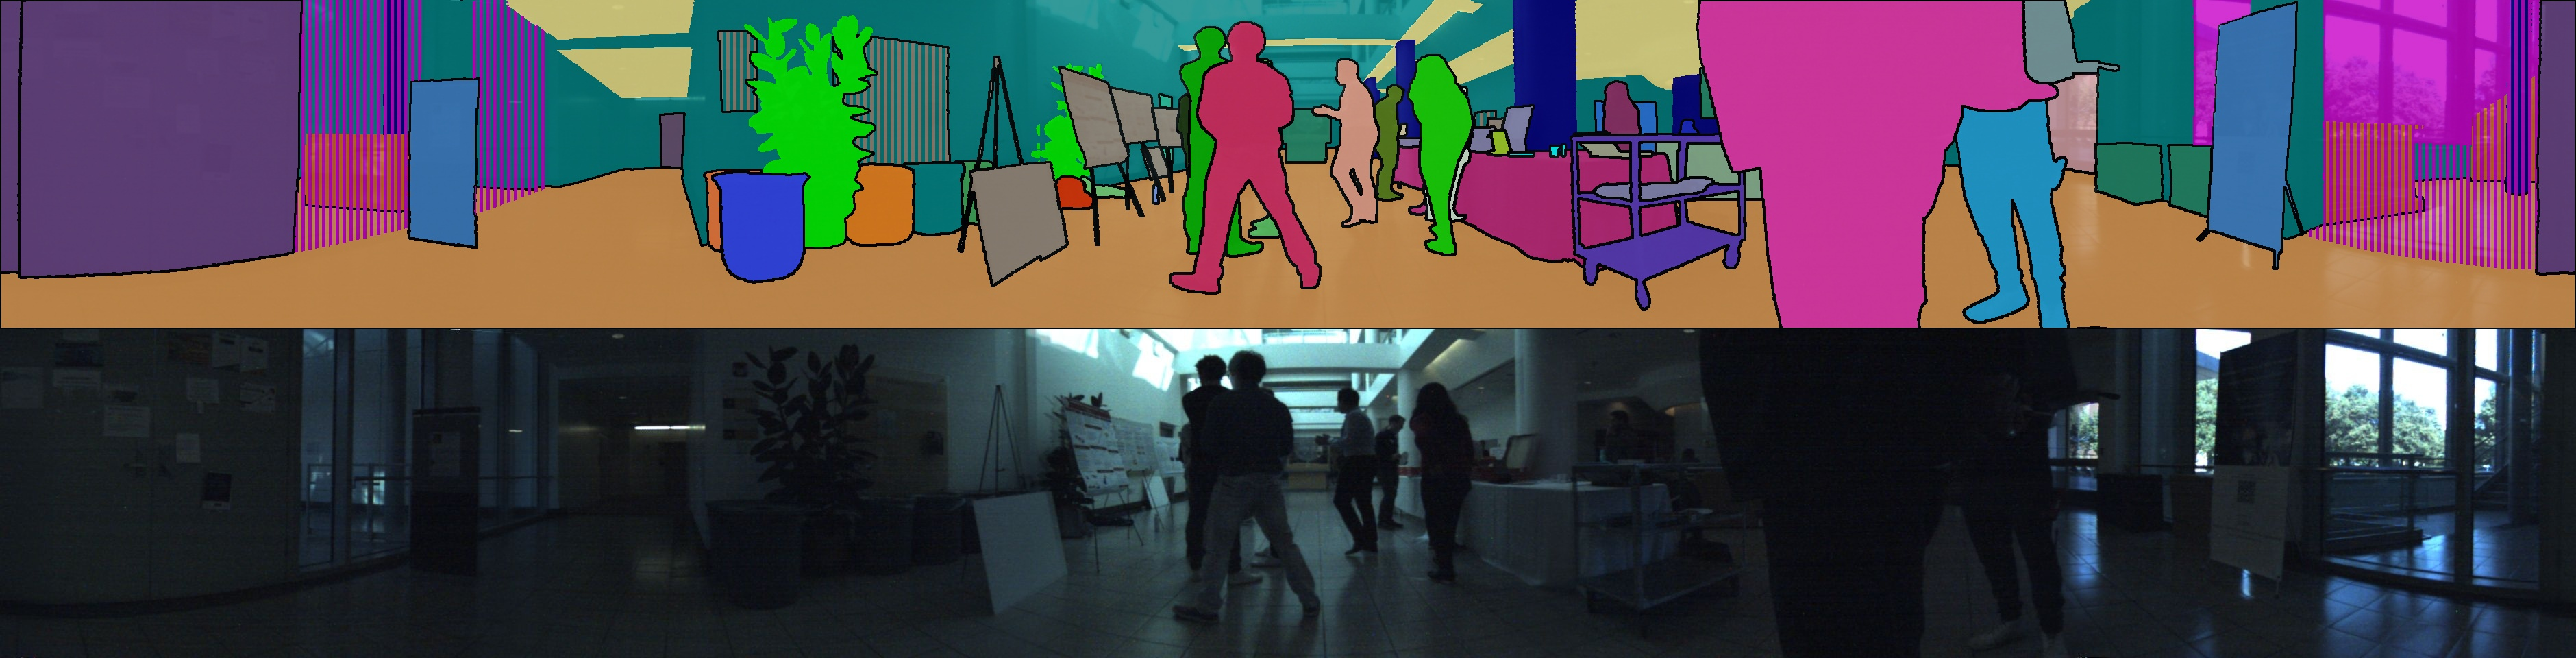}
    \includegraphics[width=\linewidth]{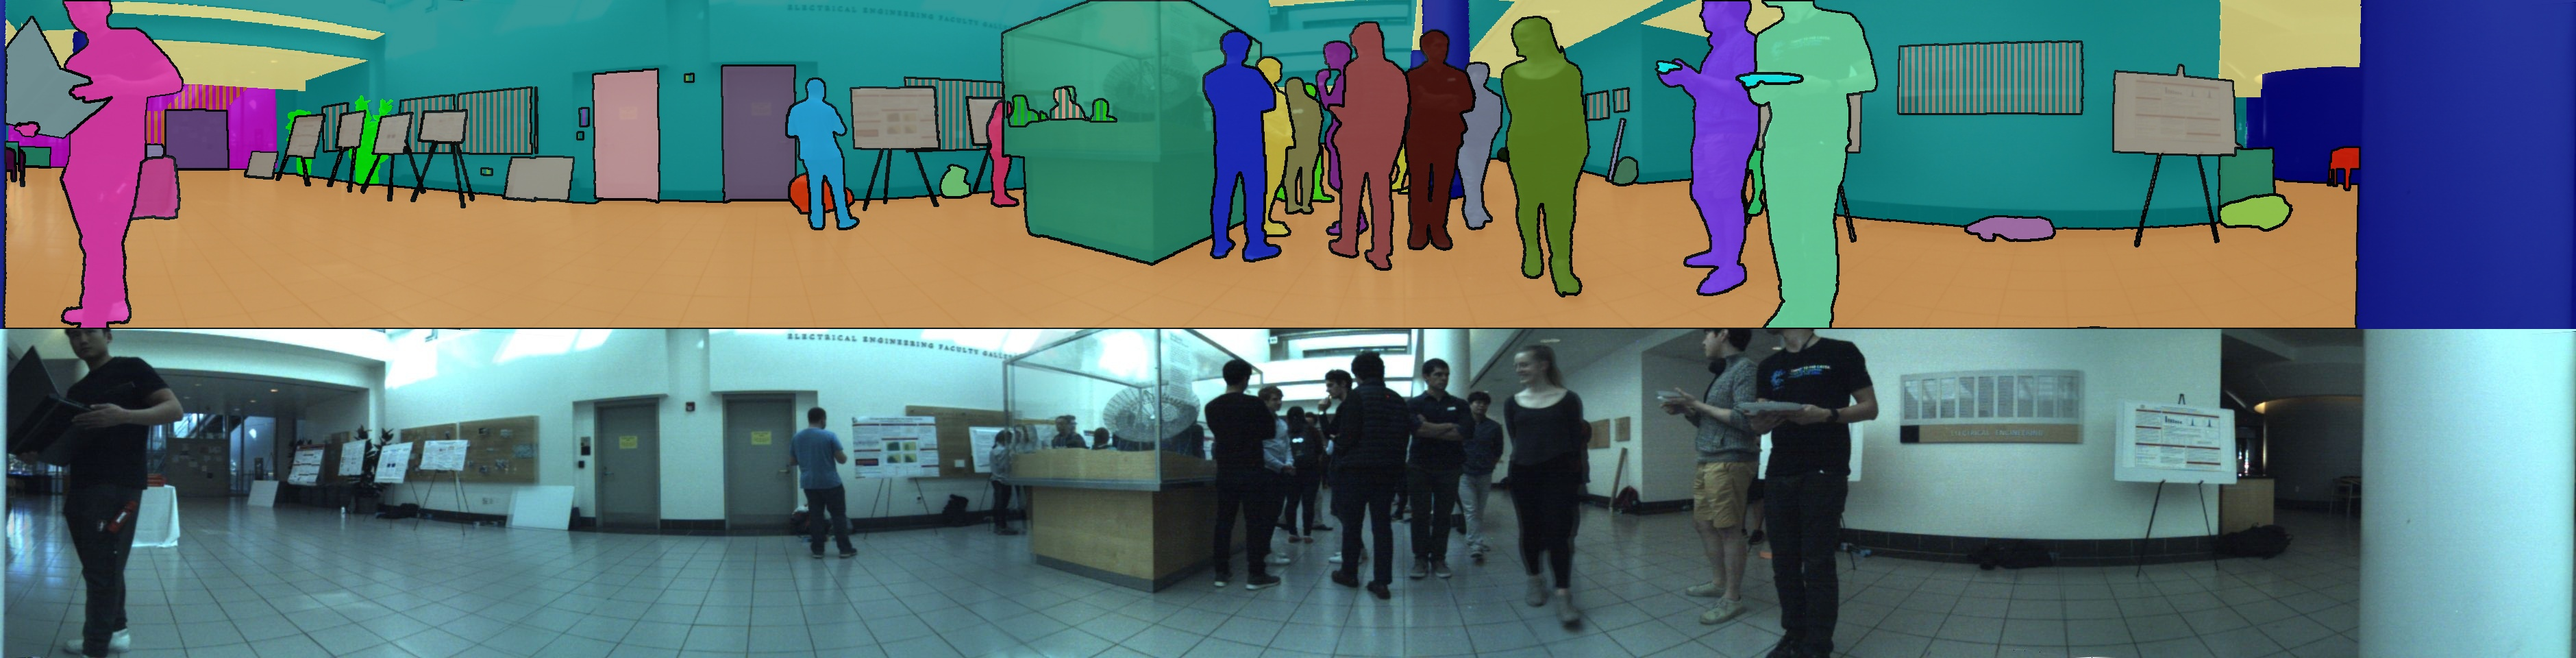}
\end{figure*}

\begin{figure*}[!ht]
    \centering
    \includegraphics[width=\linewidth]{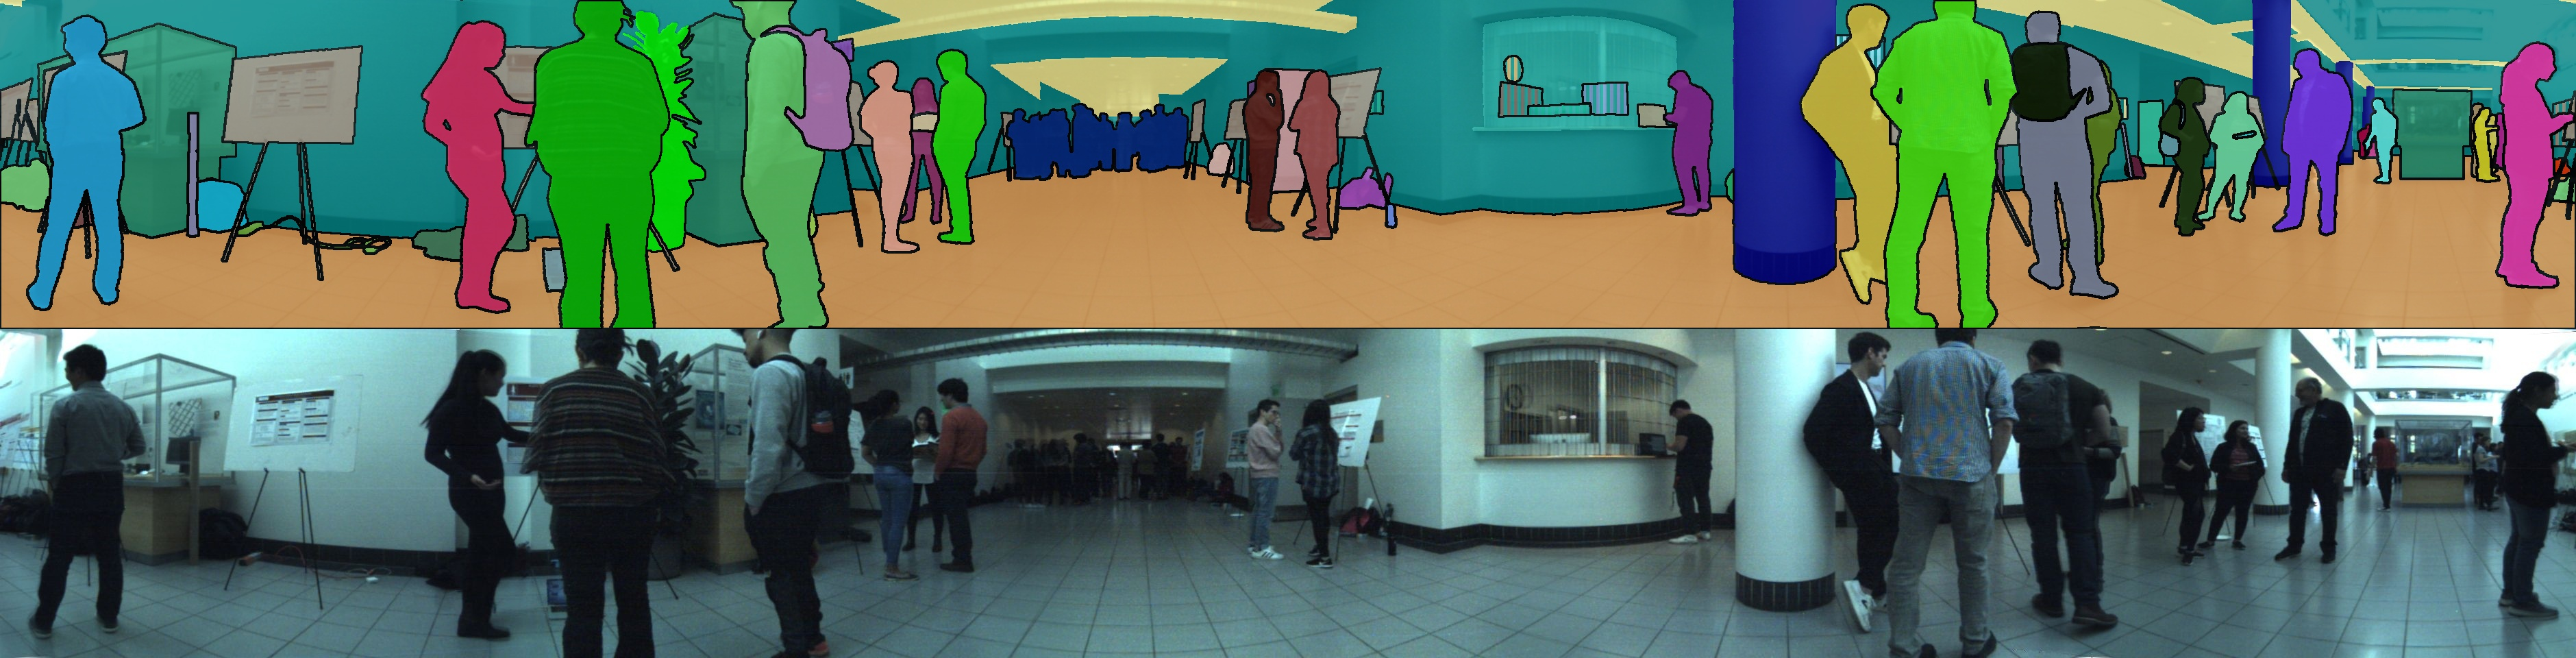}
    \includegraphics[width=\linewidth]{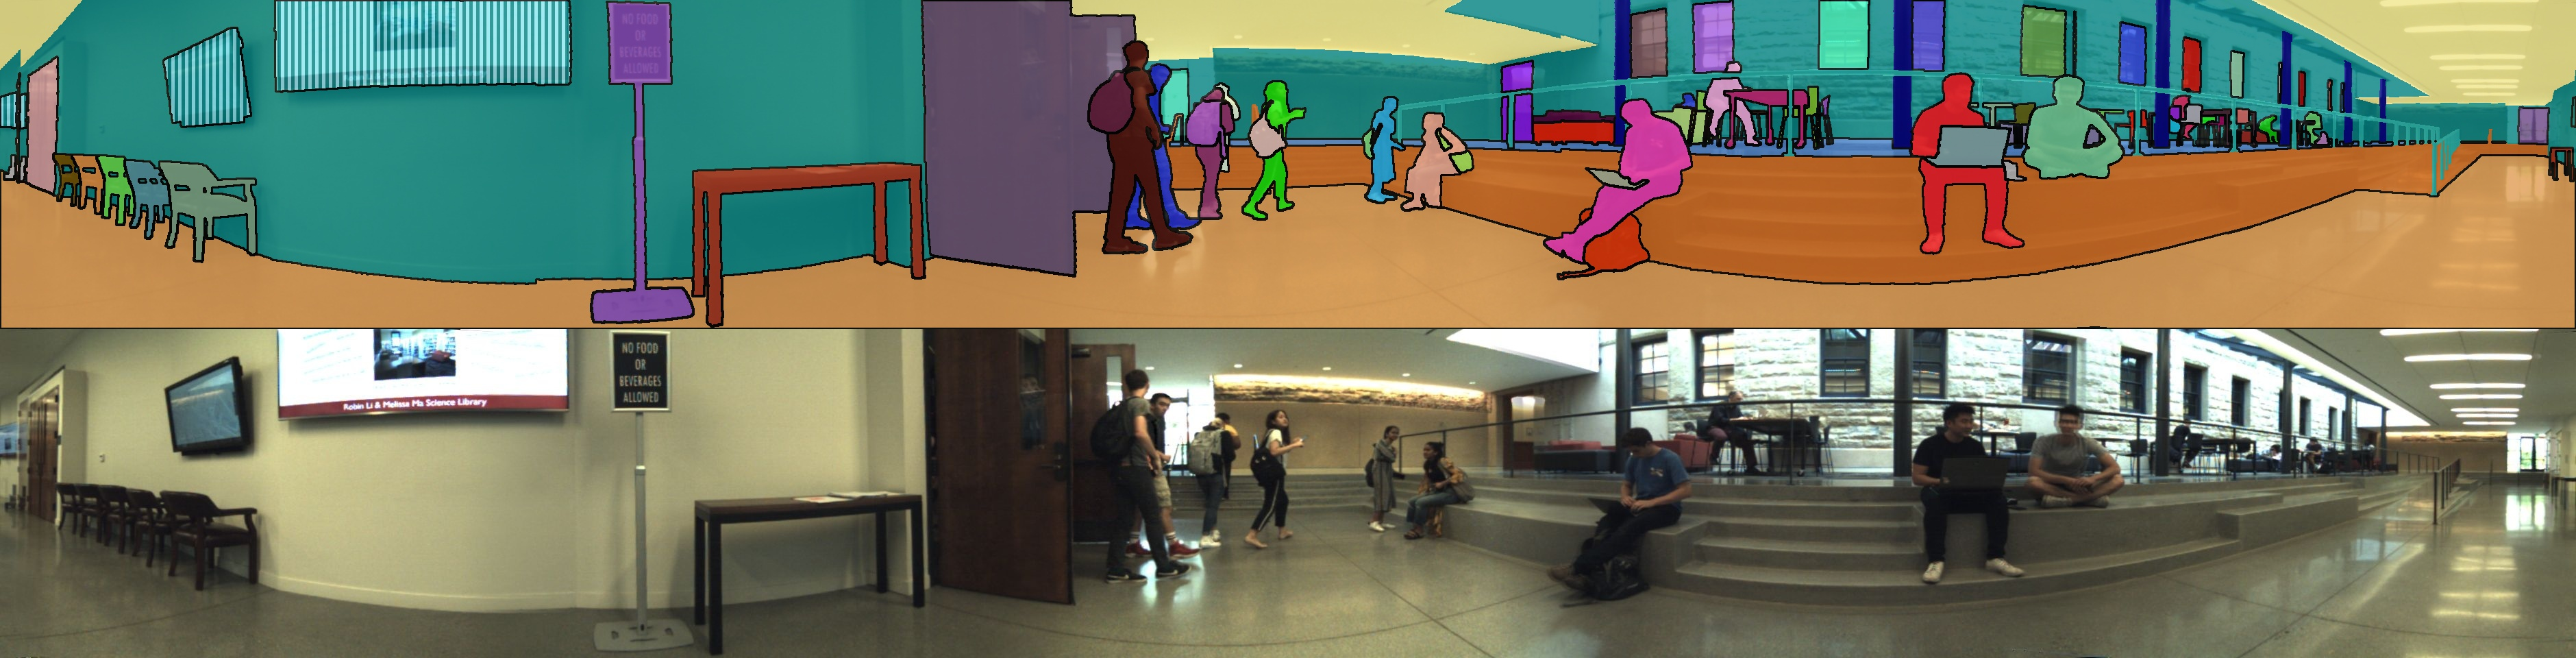}
    \includegraphics[width=\linewidth]{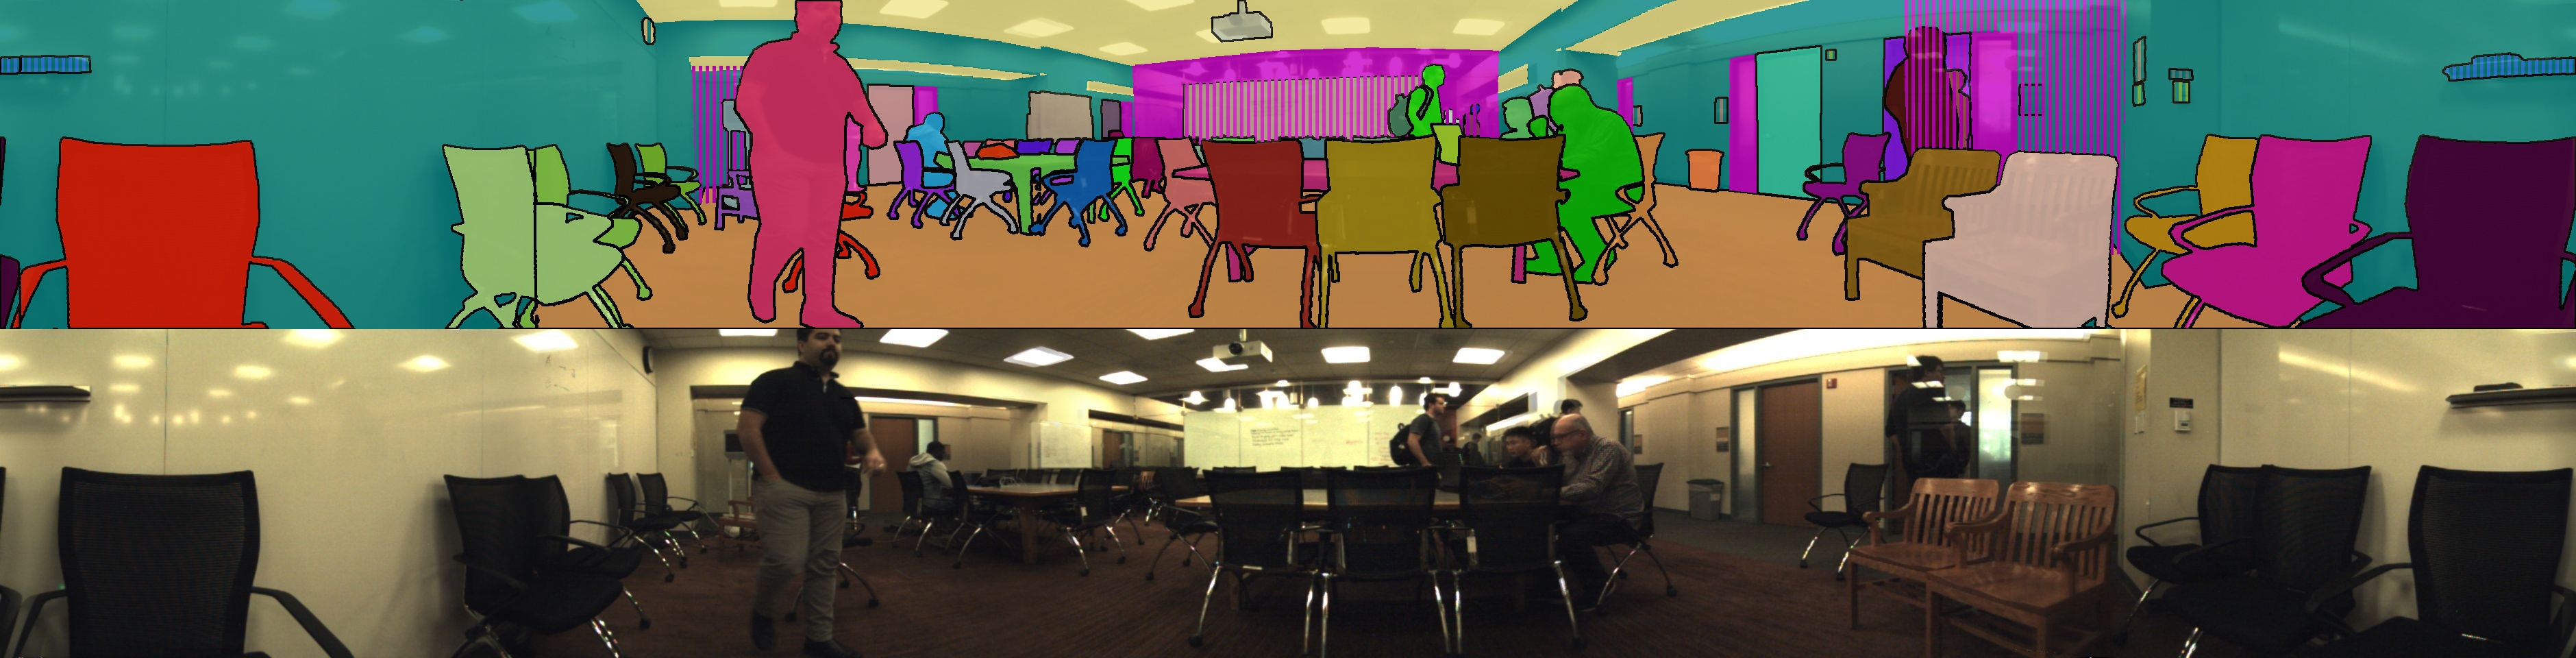}
    \includegraphics[width=\linewidth]{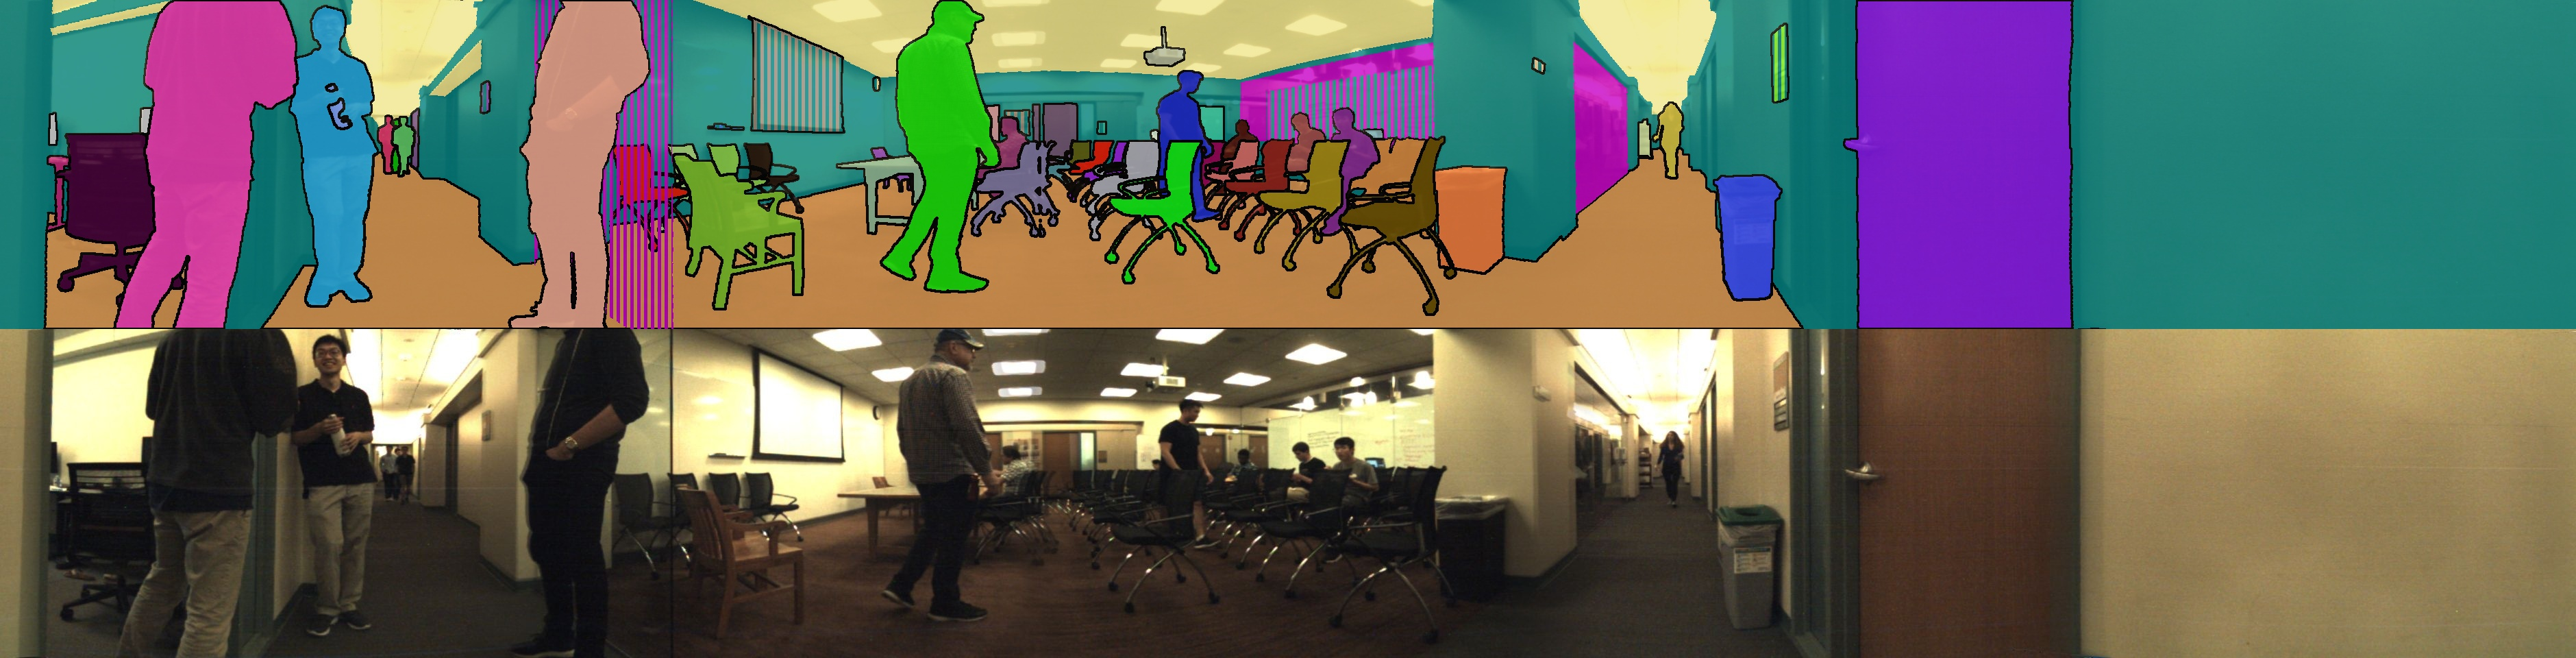}
    \includegraphics[width=\linewidth]{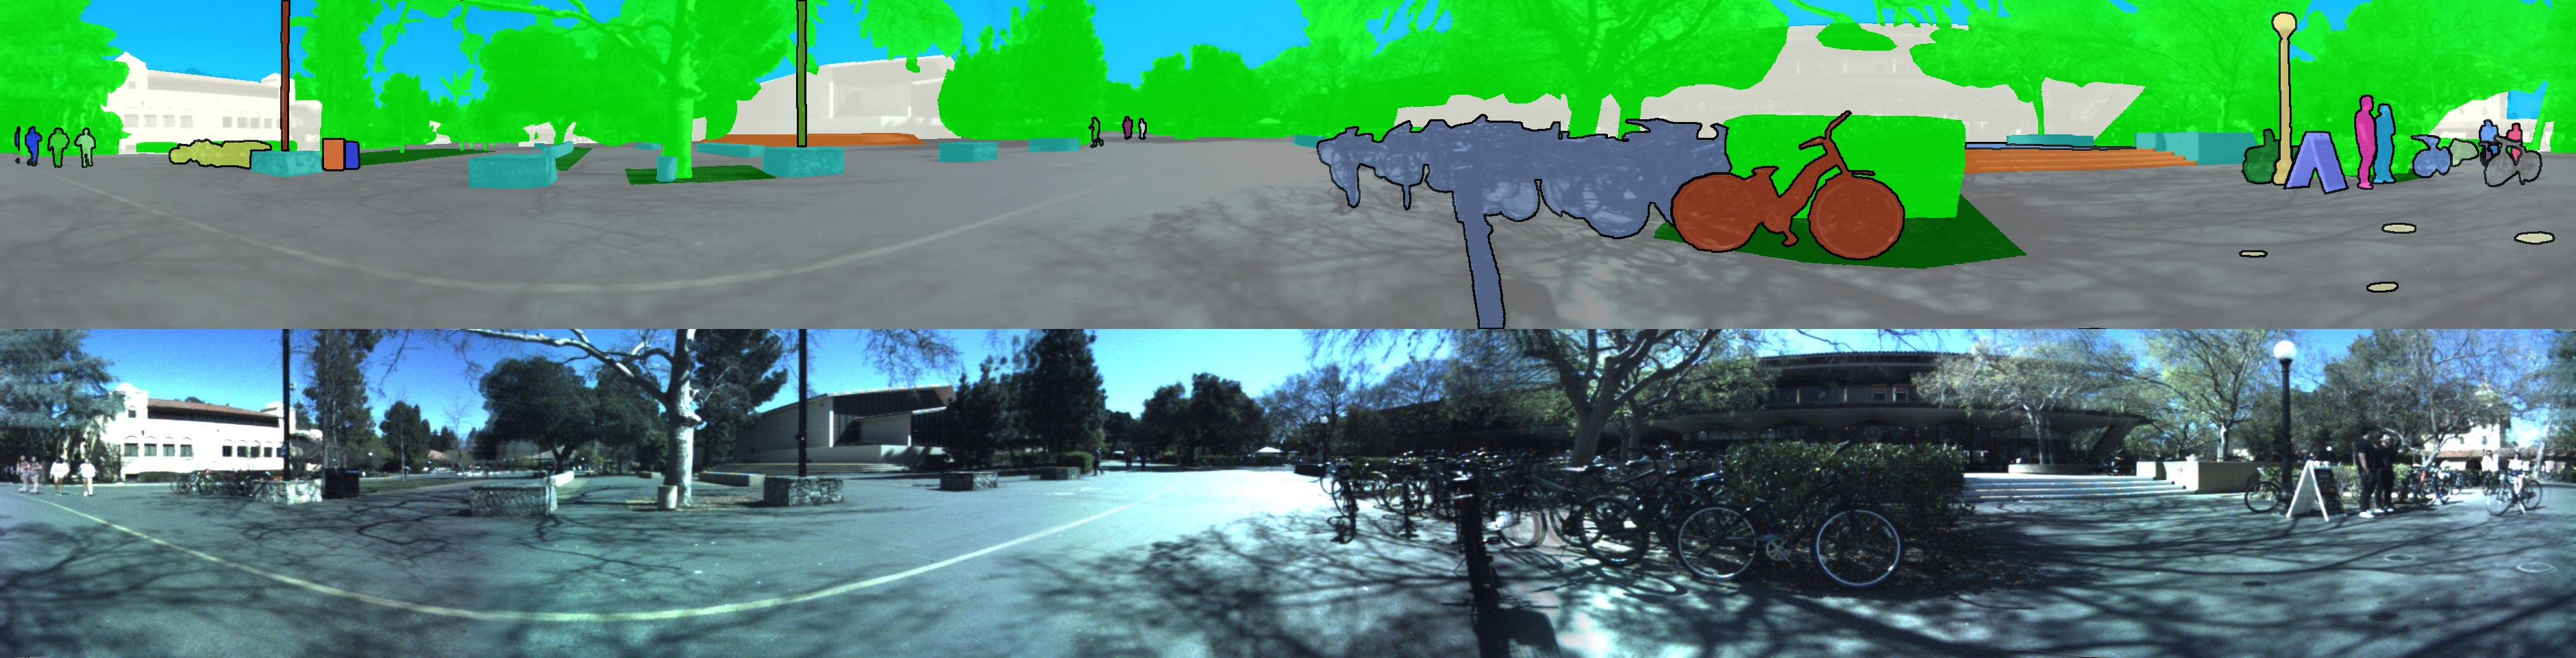}
\end{figure*}

\begin{figure*}[!ht]
    \centering
    \includegraphics[width=\linewidth]{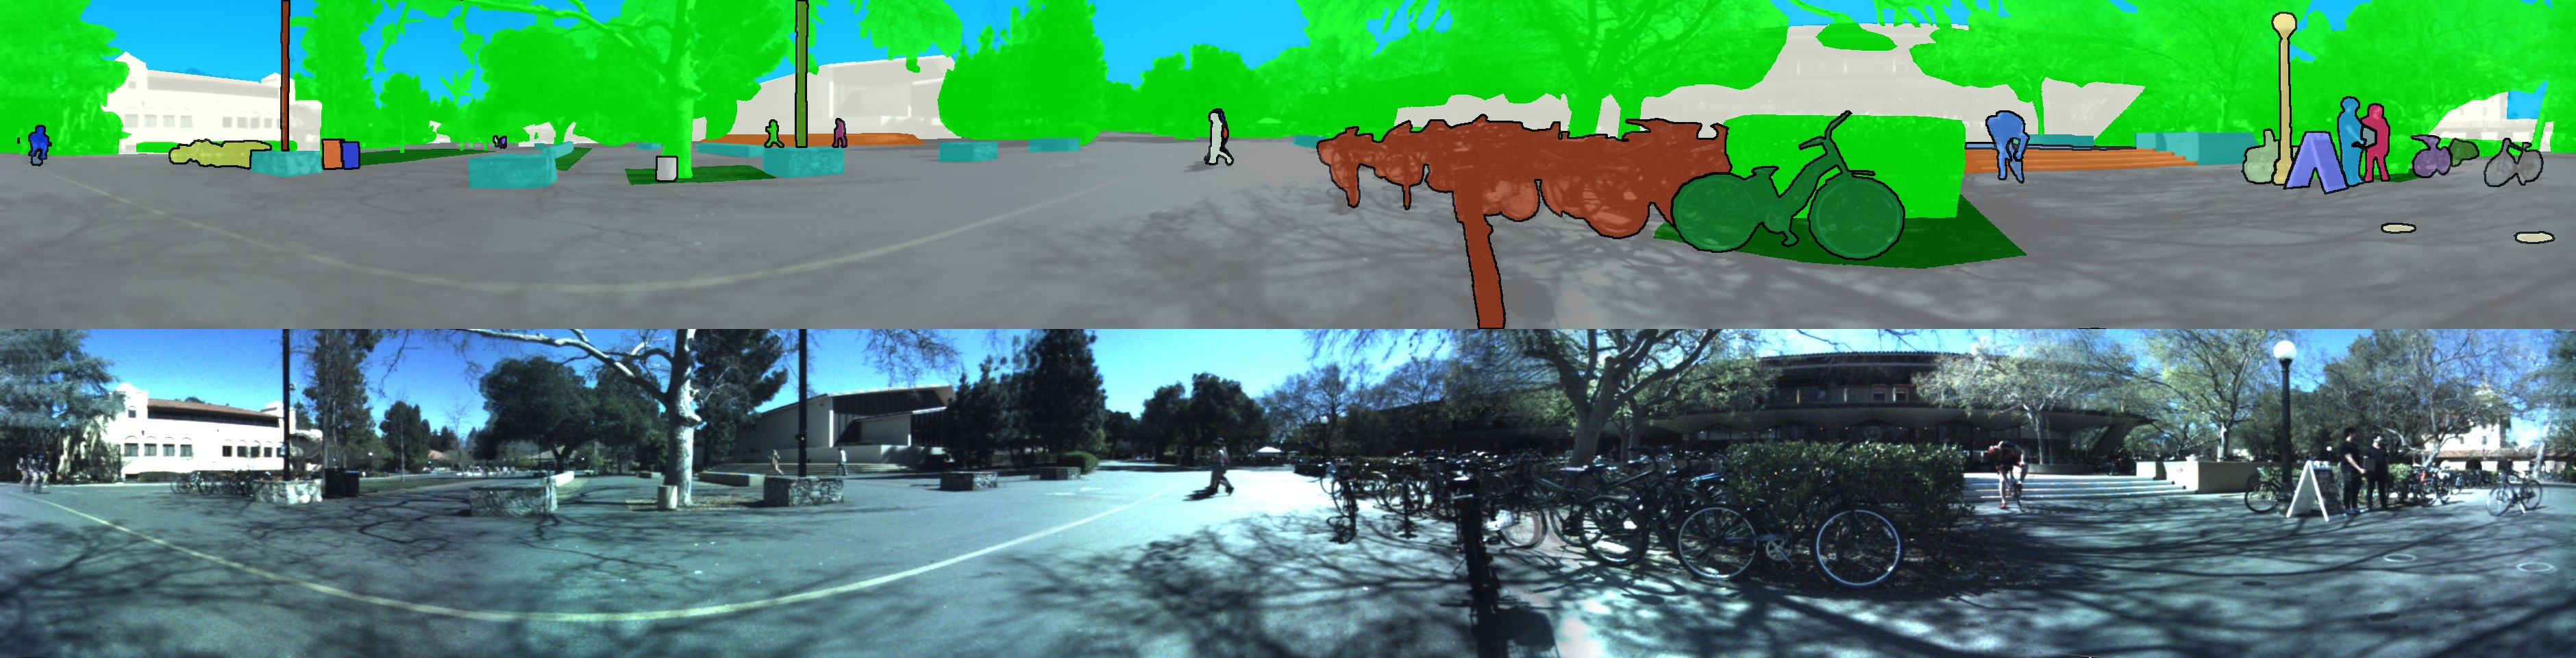}
    \includegraphics[width=\linewidth]{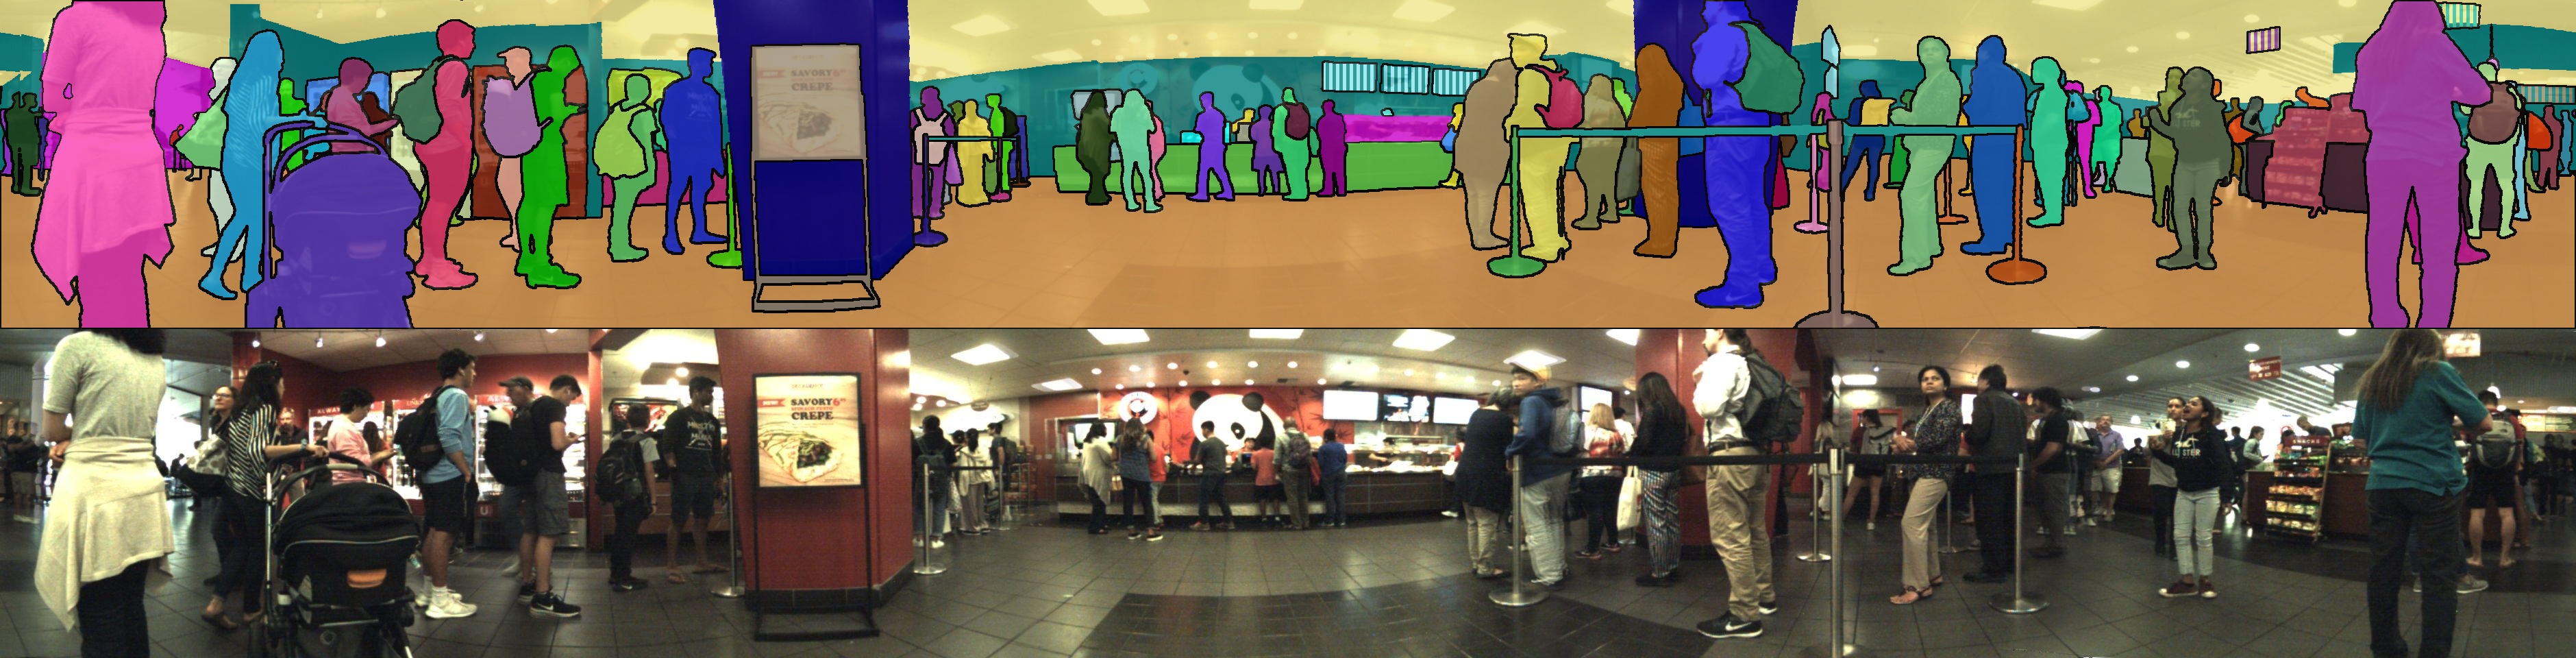}
    \includegraphics[width=\linewidth]{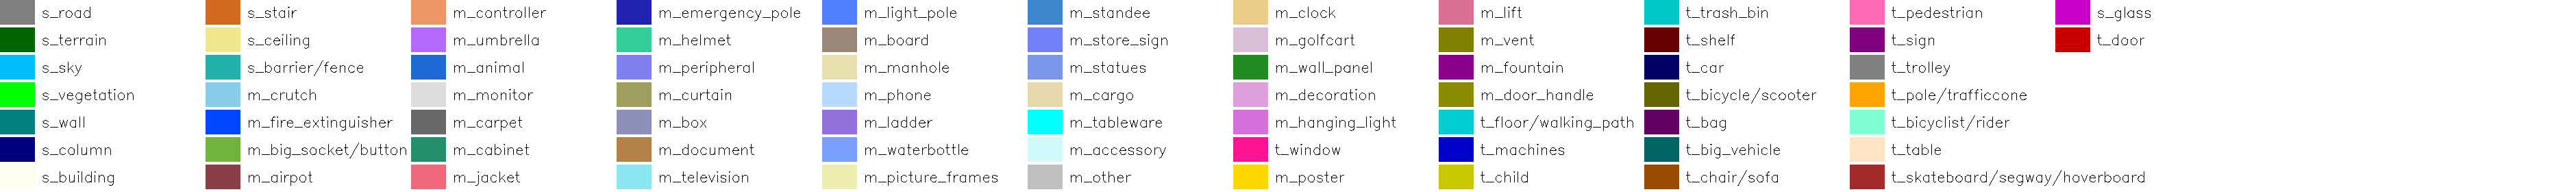}
    \caption{Visualization of JRDB-PanoTrack panoptic segmentation annotations.
    %from each of the 27 training sequences. Each sequence is represented by two images: one displaying 2D panoptic segmentation labels and the other depicting the corresponding original scene. 
    The images showcase diverse settings, ranging from indoor to outdoor environments, characterized by different lighting conditions, varied levels of human clutter, and dynamic activities. Featured locations include a variety of indoor and outdoor spaces, such as roads, malls, sidewalks, restaurants, plazas, parks, halls, classrooms, laboratories, and office buildings.
    Meanwhile, we label different floors and objects behind the glass (striped areas) different floors for better real-world robot navigation, human-robot interaction and decision.}
    \label{fig:stacked_images}
\end{figure*}
